# Supplementary material for: Local Equivalence Classes of Distance-Hereditary Graphs using Split Decompositions
Source: arXiv:2602.23825 source file (2026-02-27)
Supplement: Supplementary file 1 [file Appendix_Complete_k-Partite_and_Clique-Star_QASST_Structure.pdf]

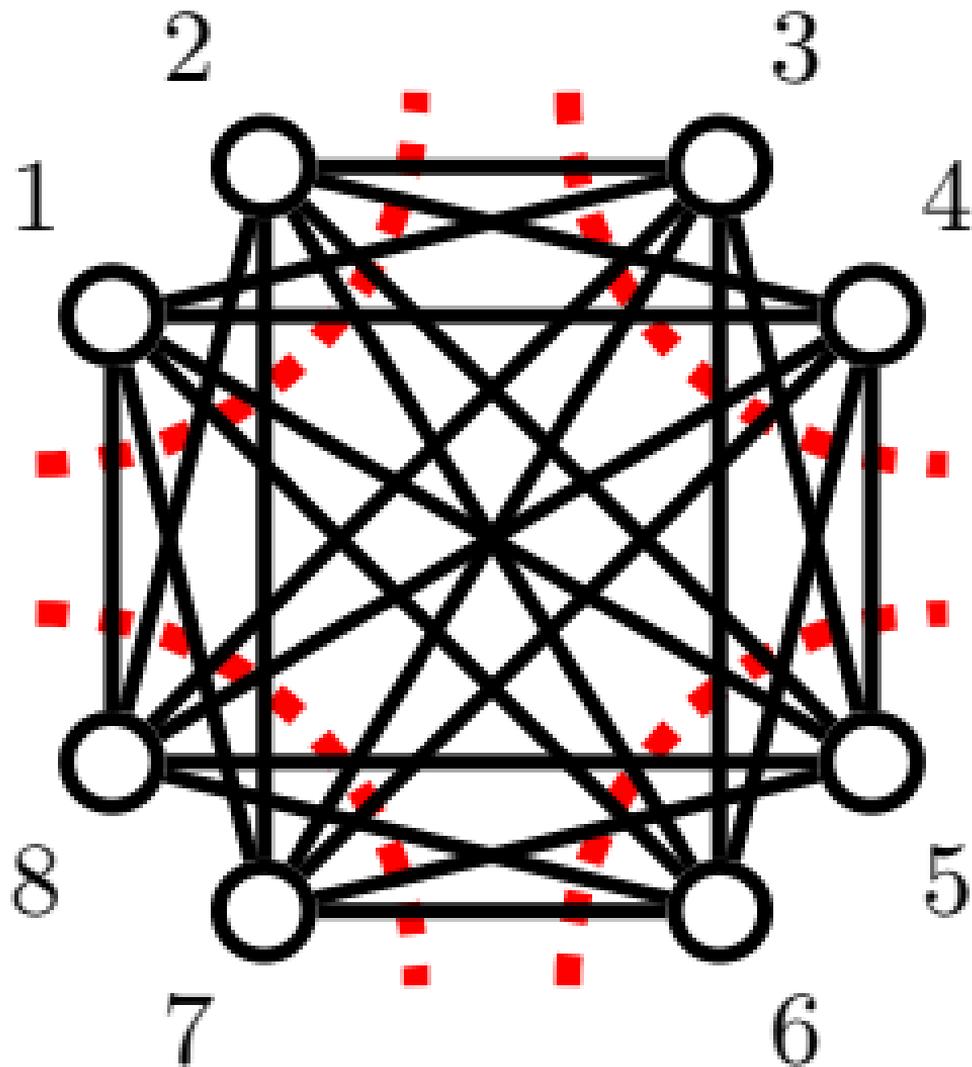

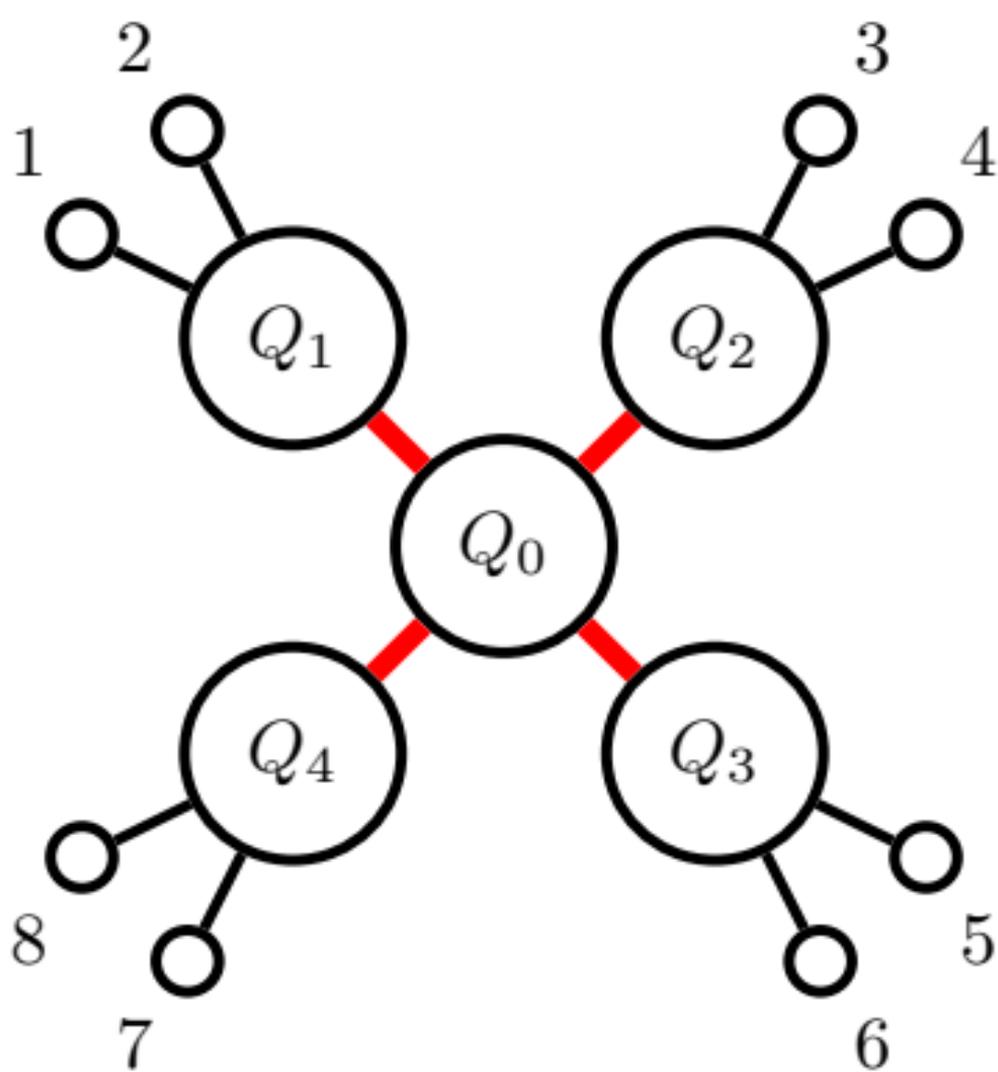

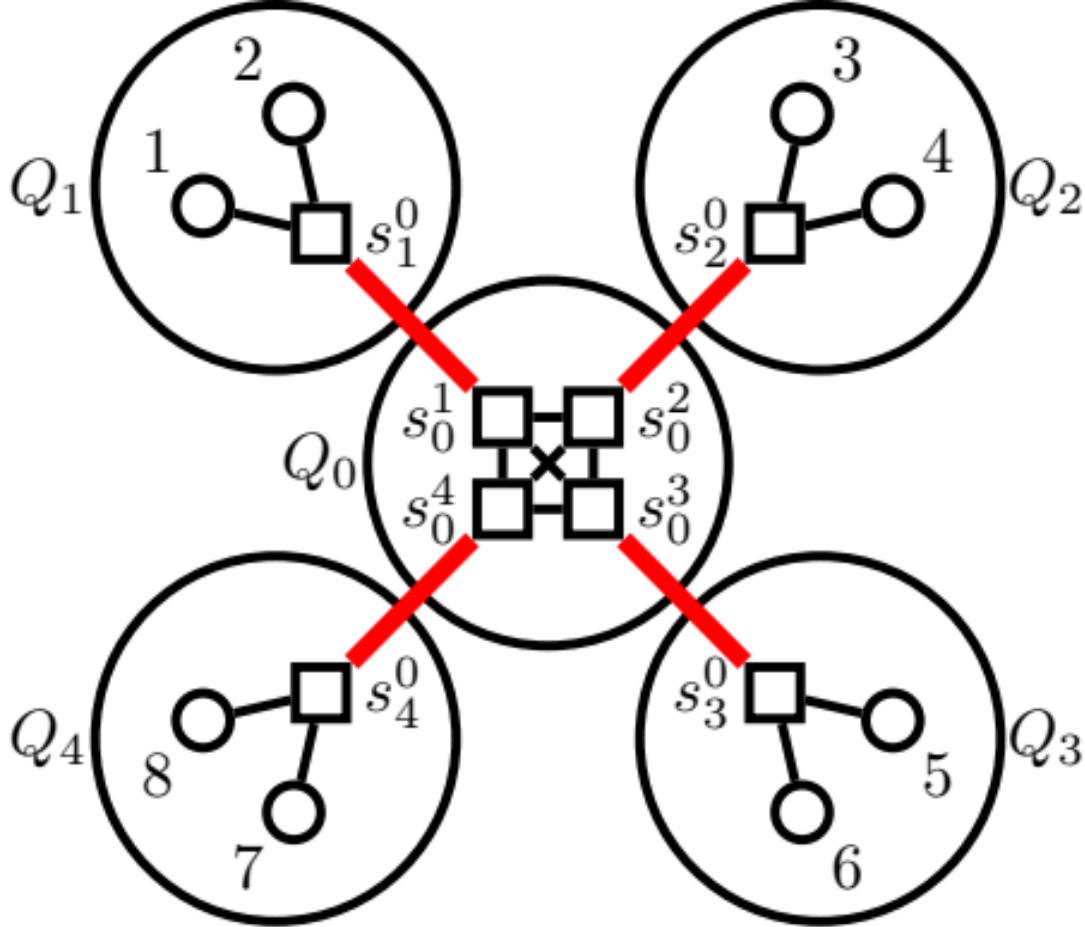

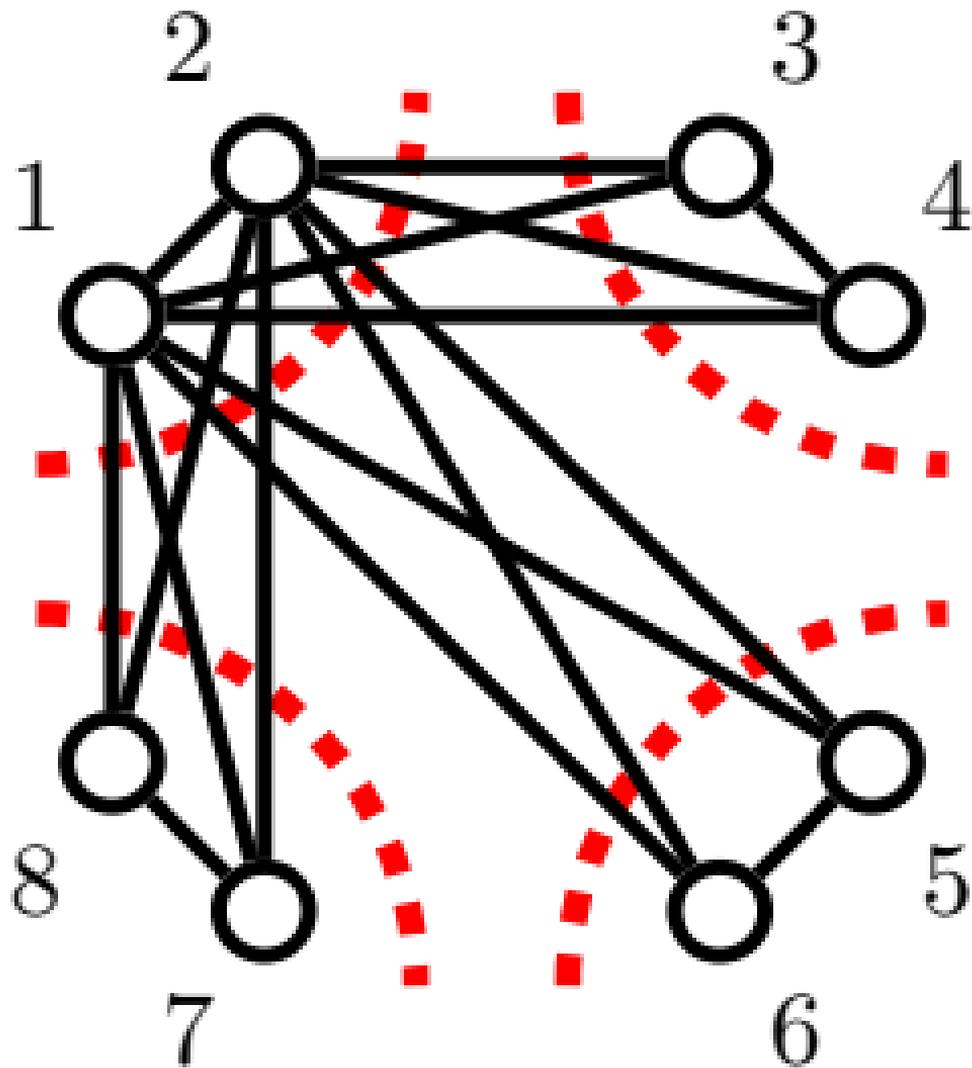

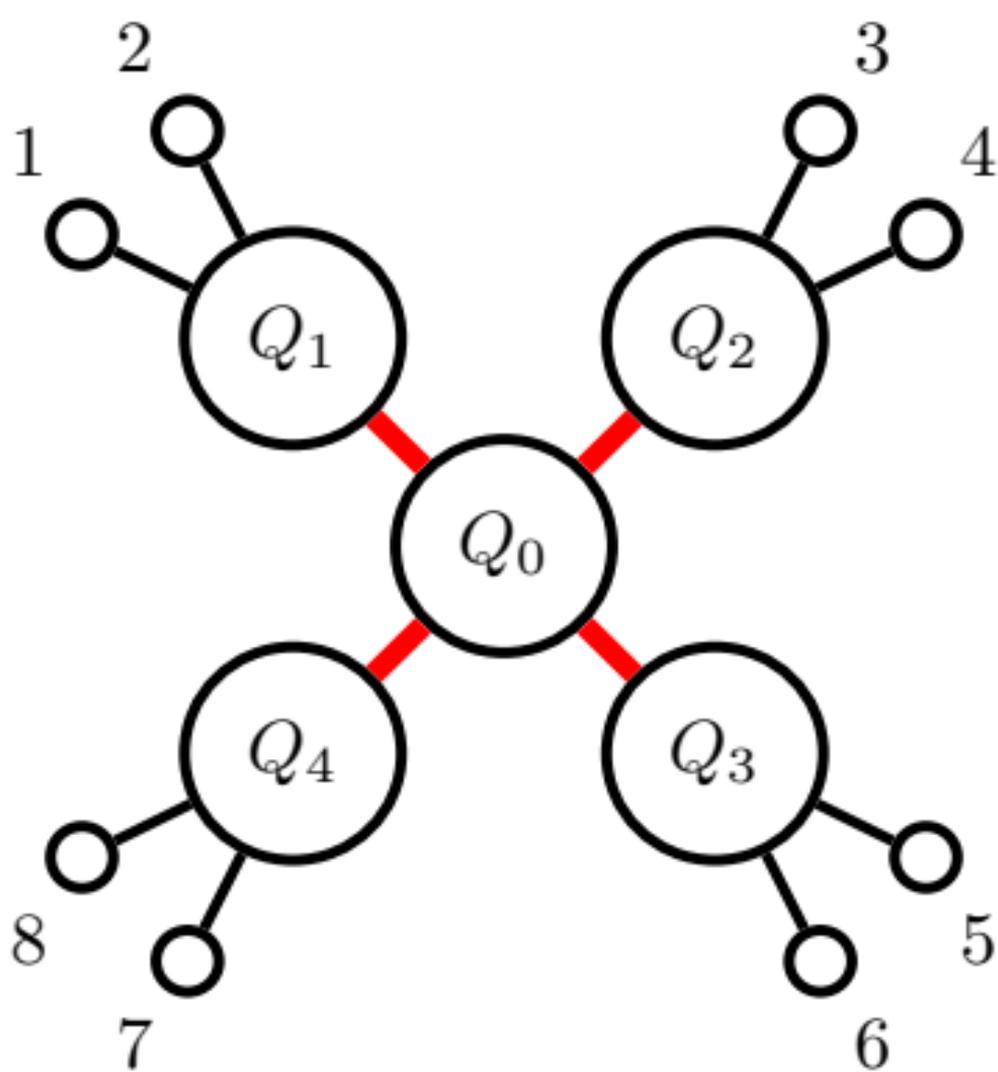

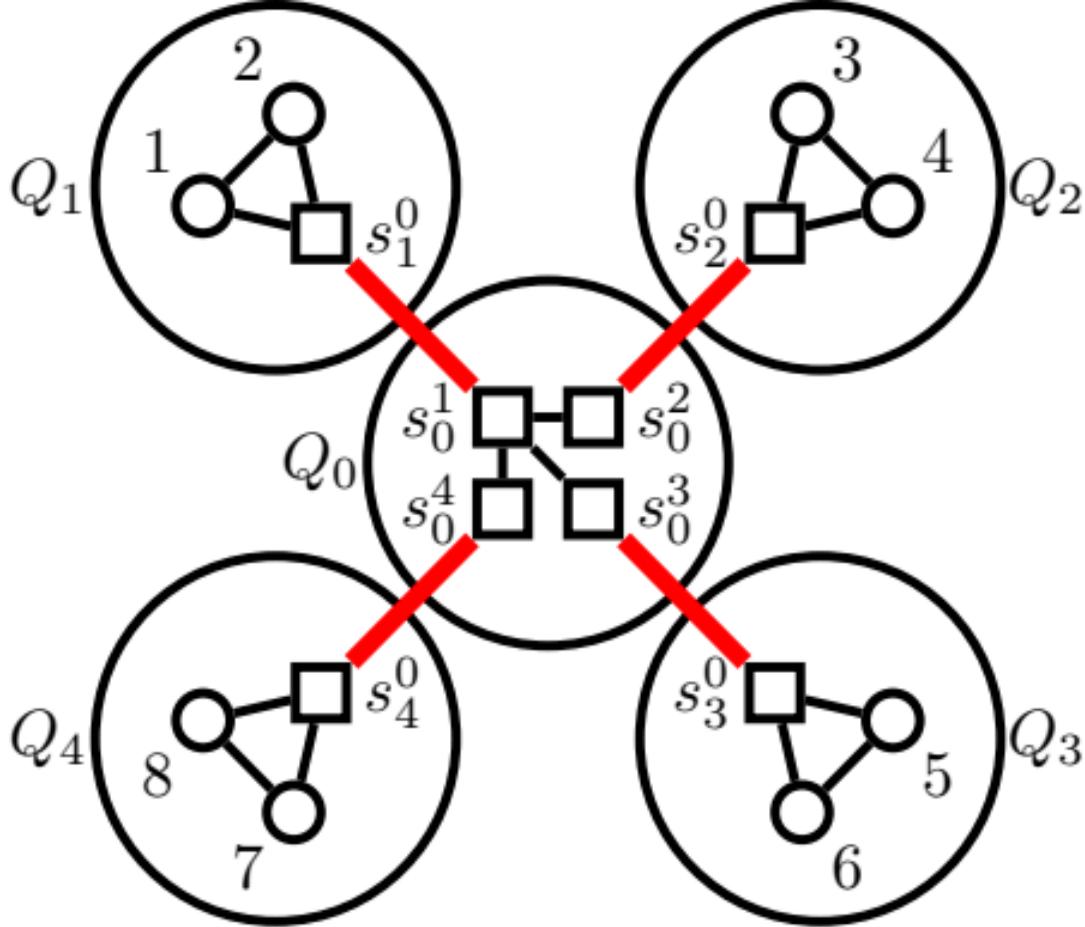

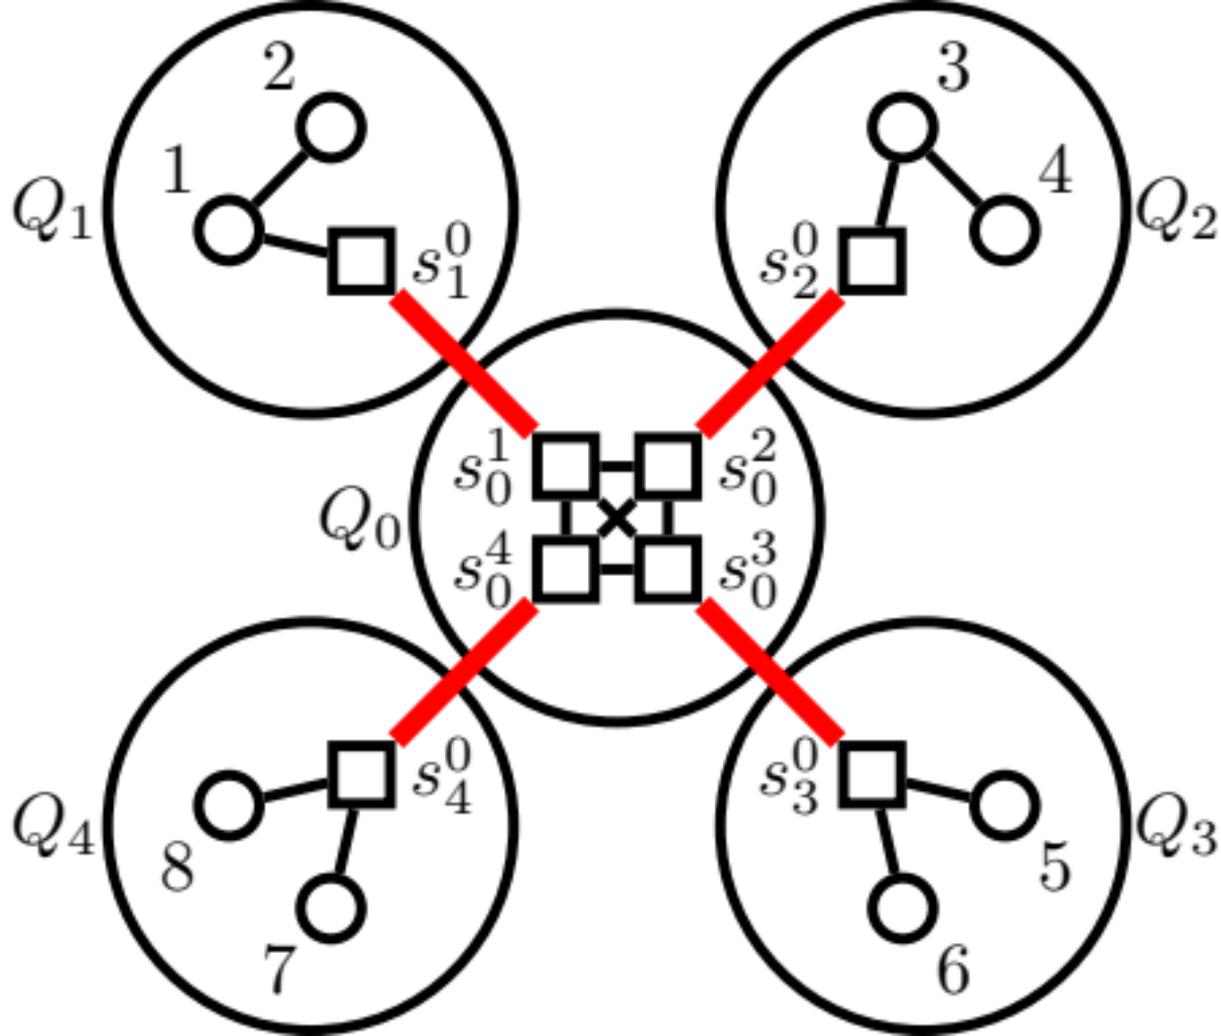

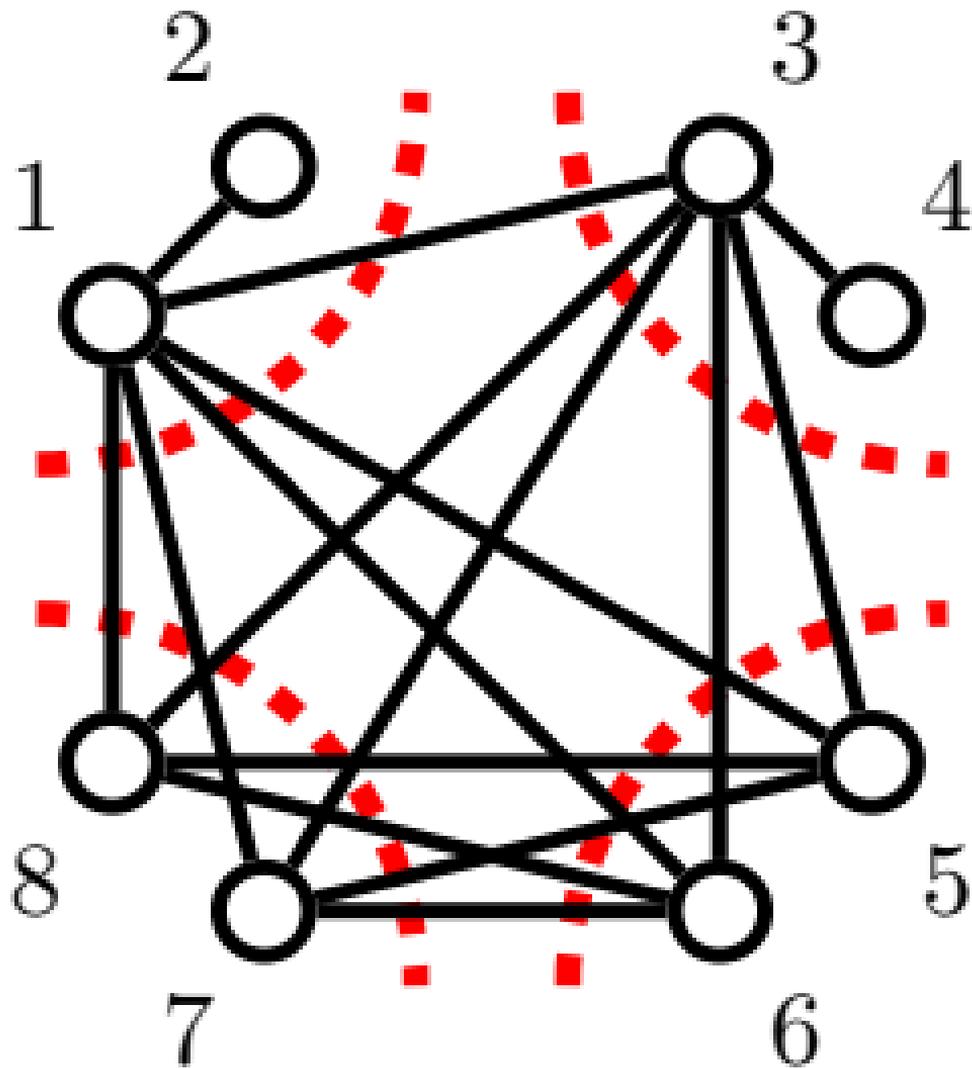

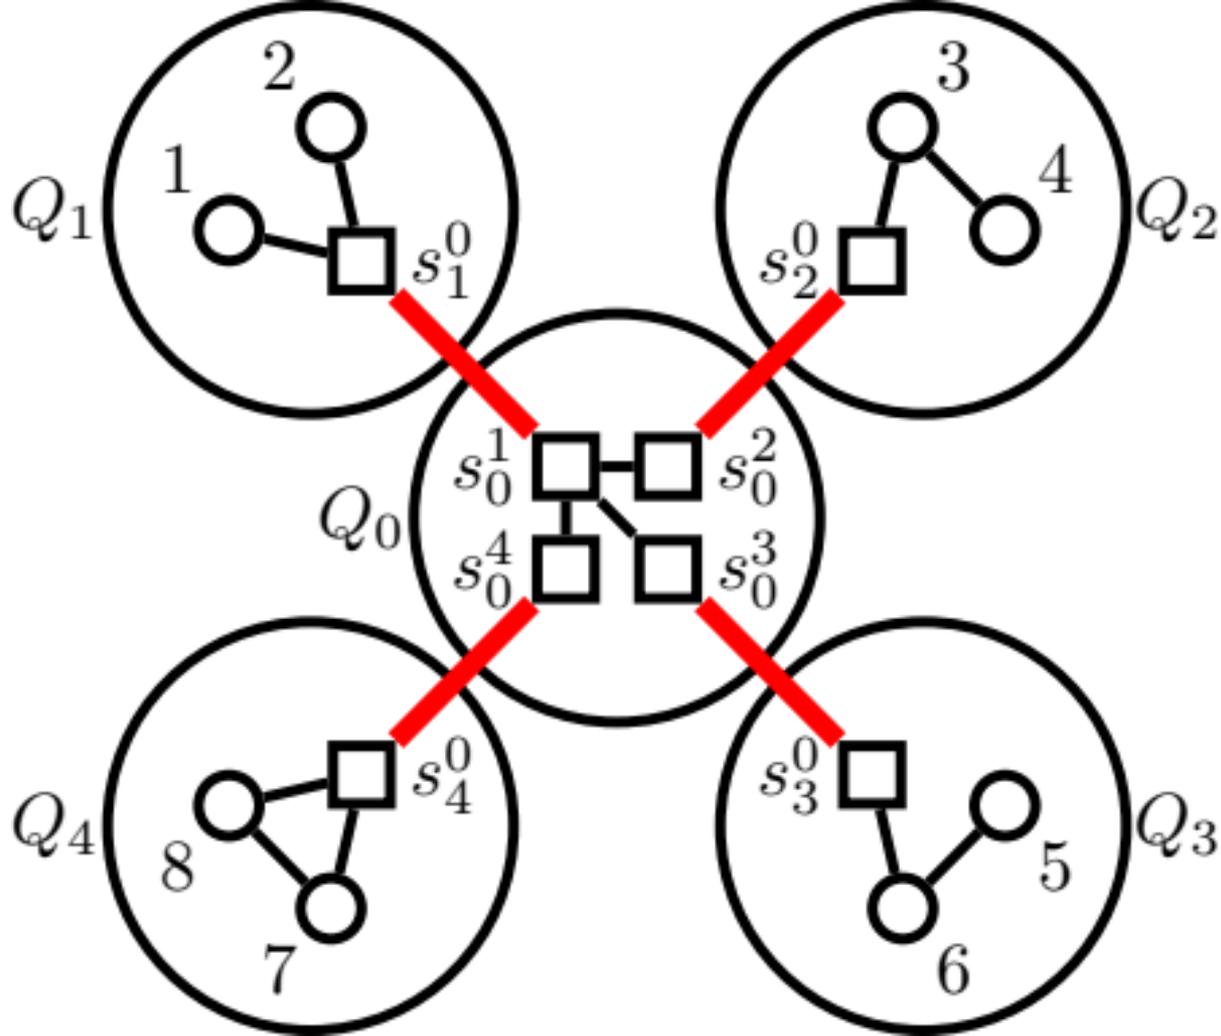

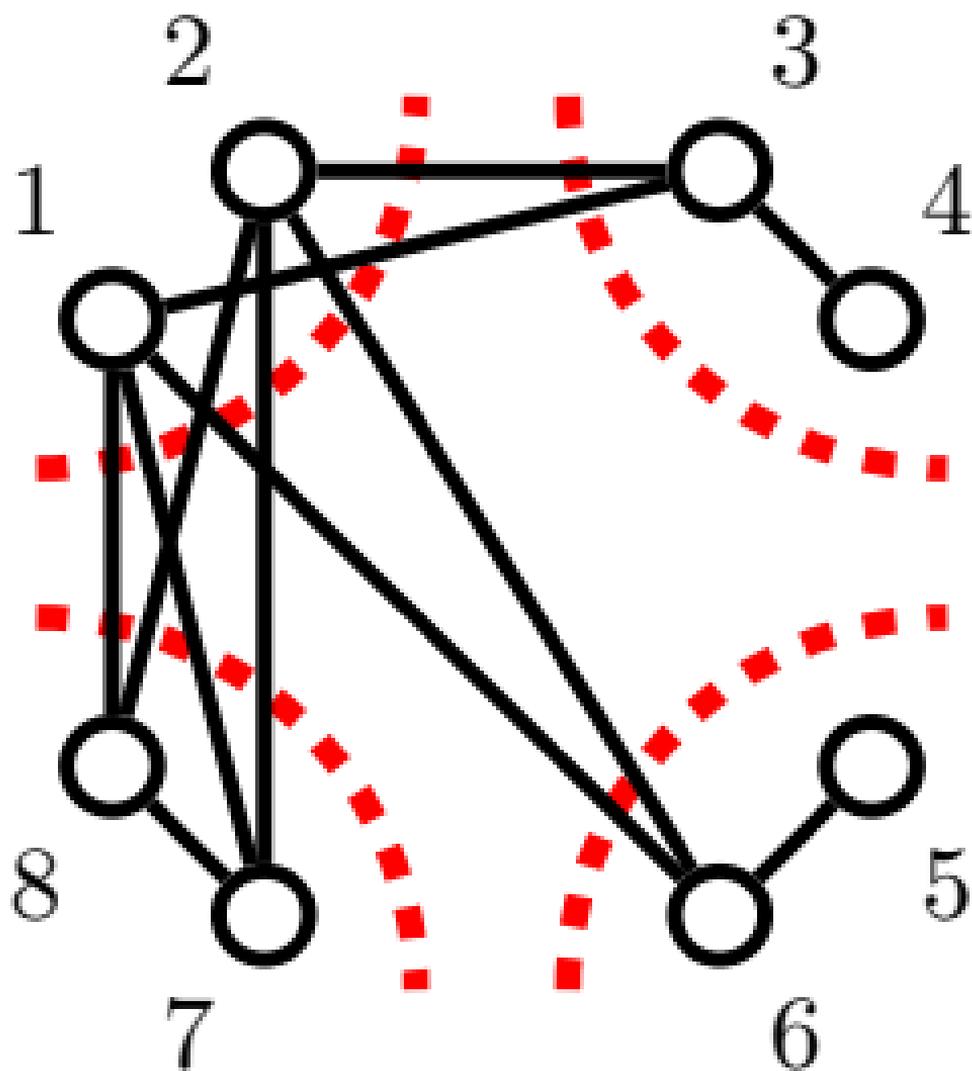

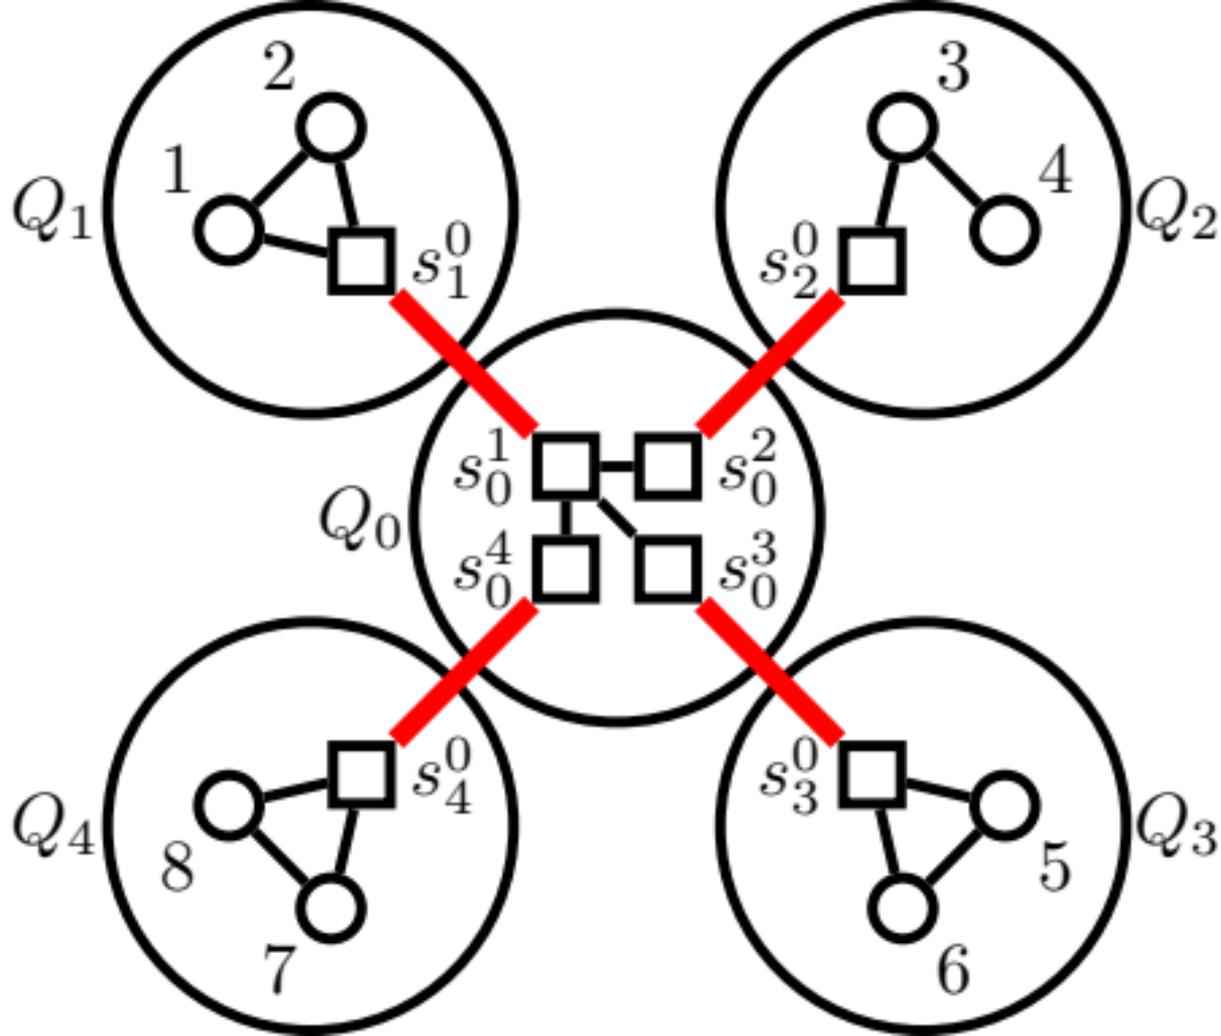

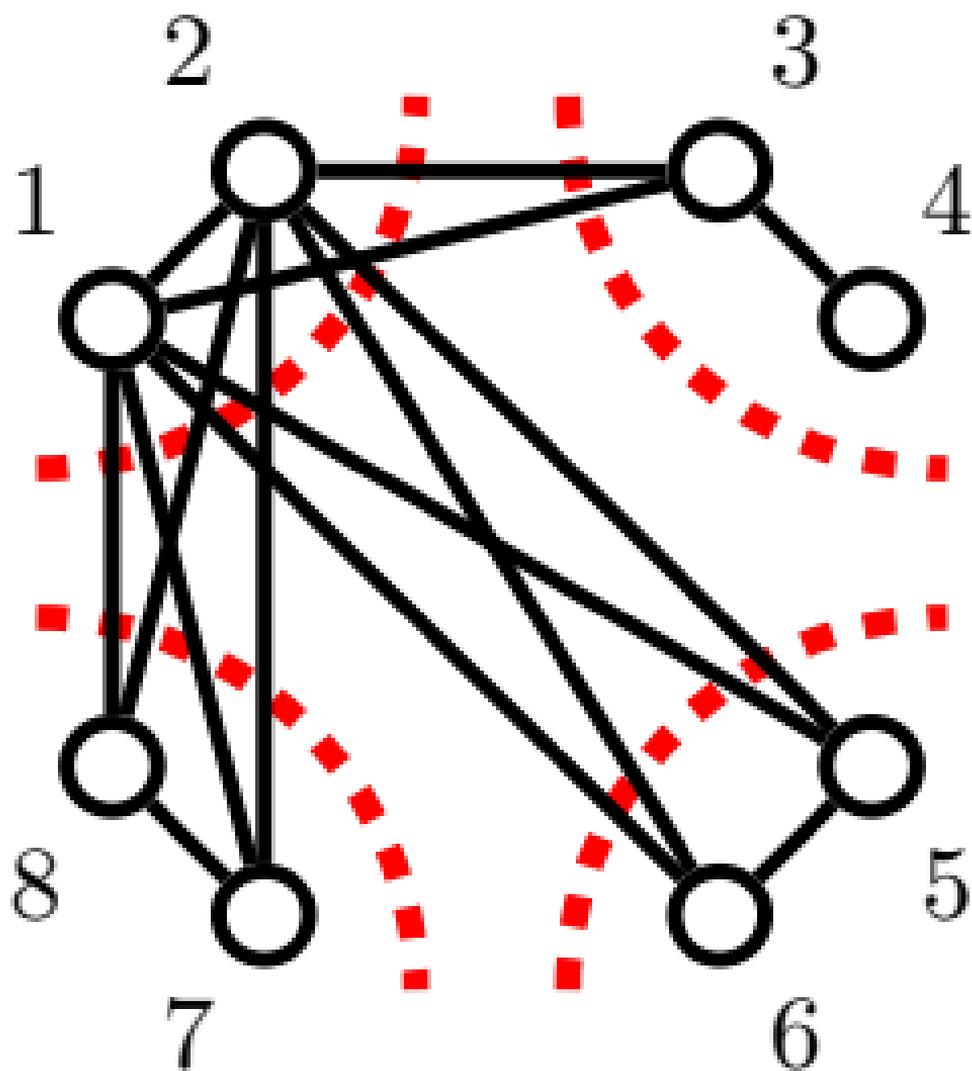

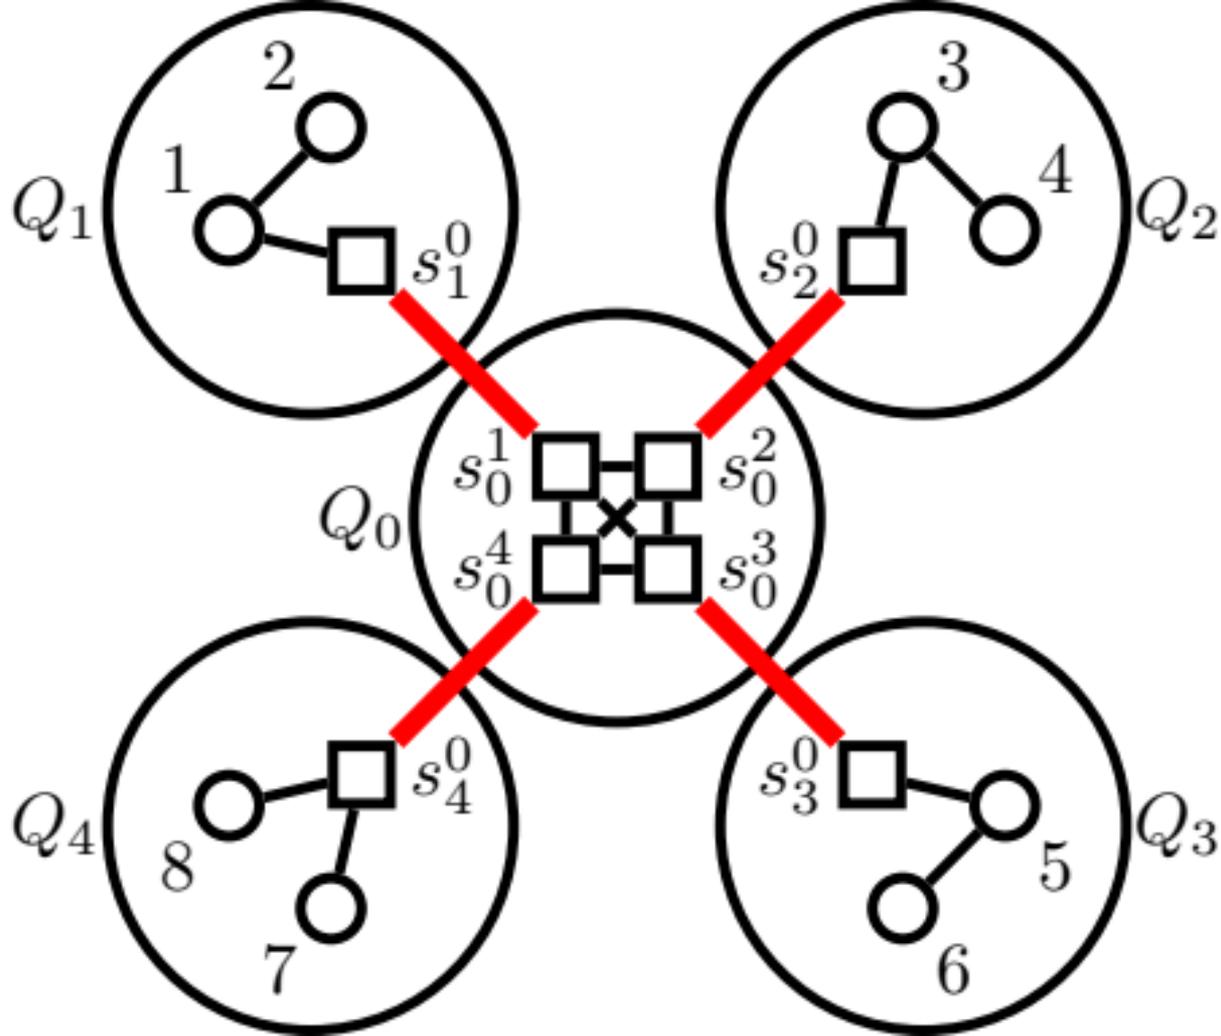

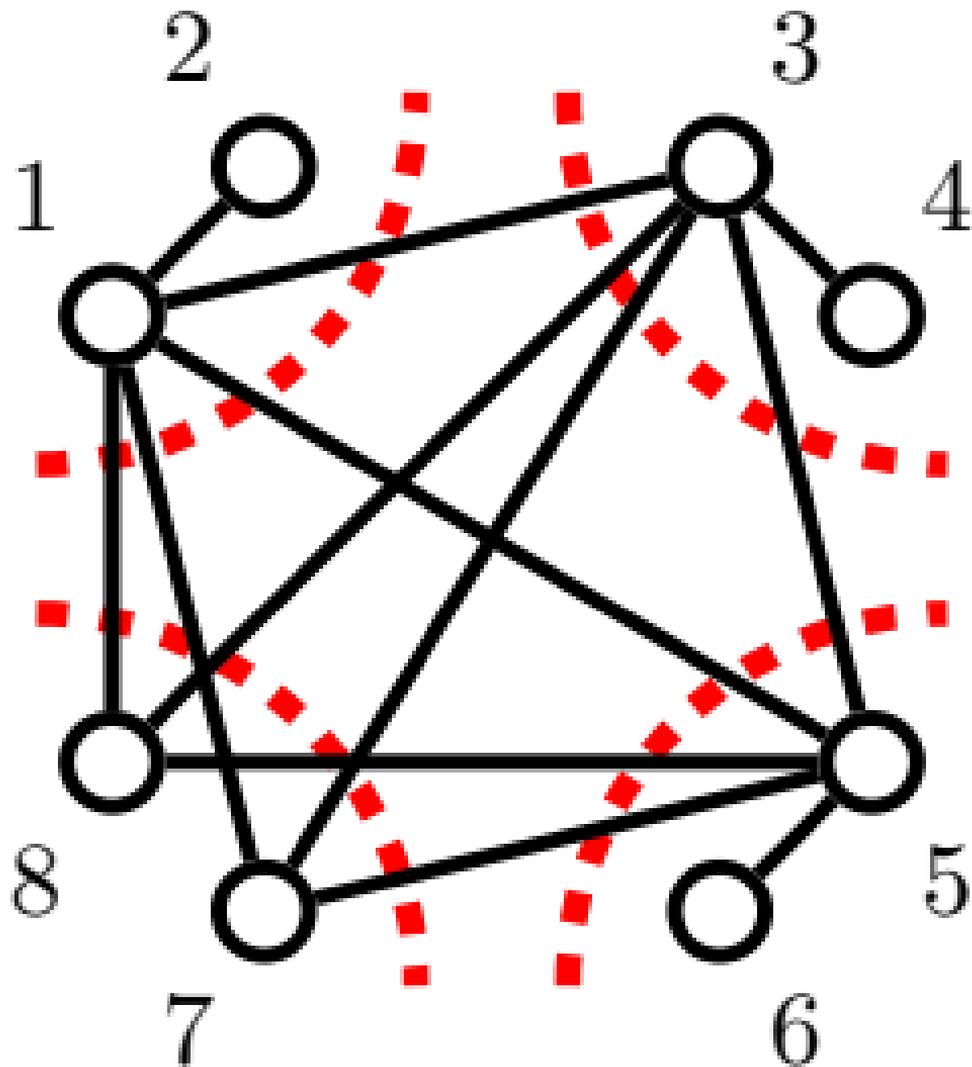

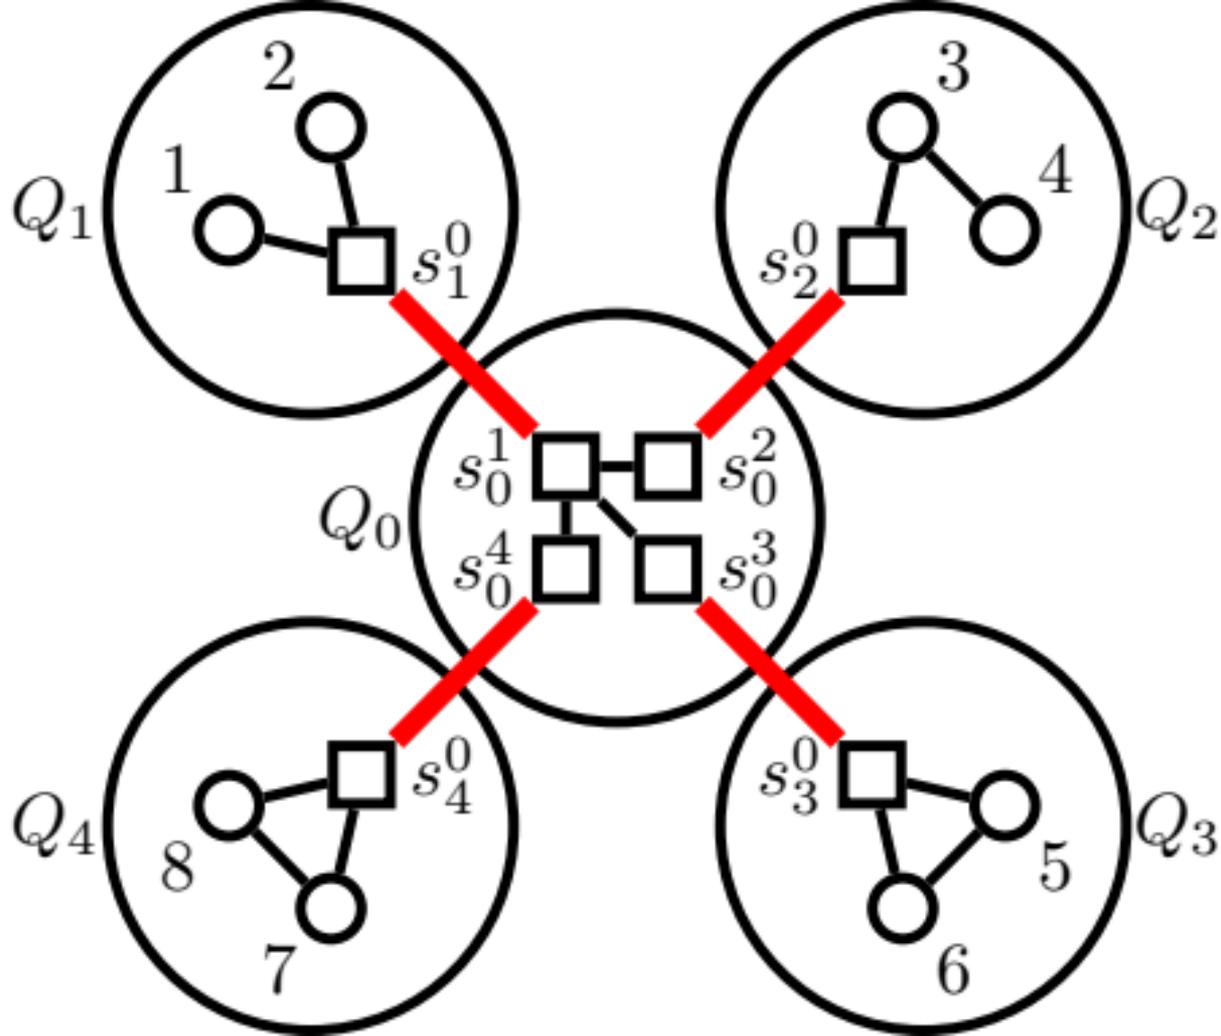

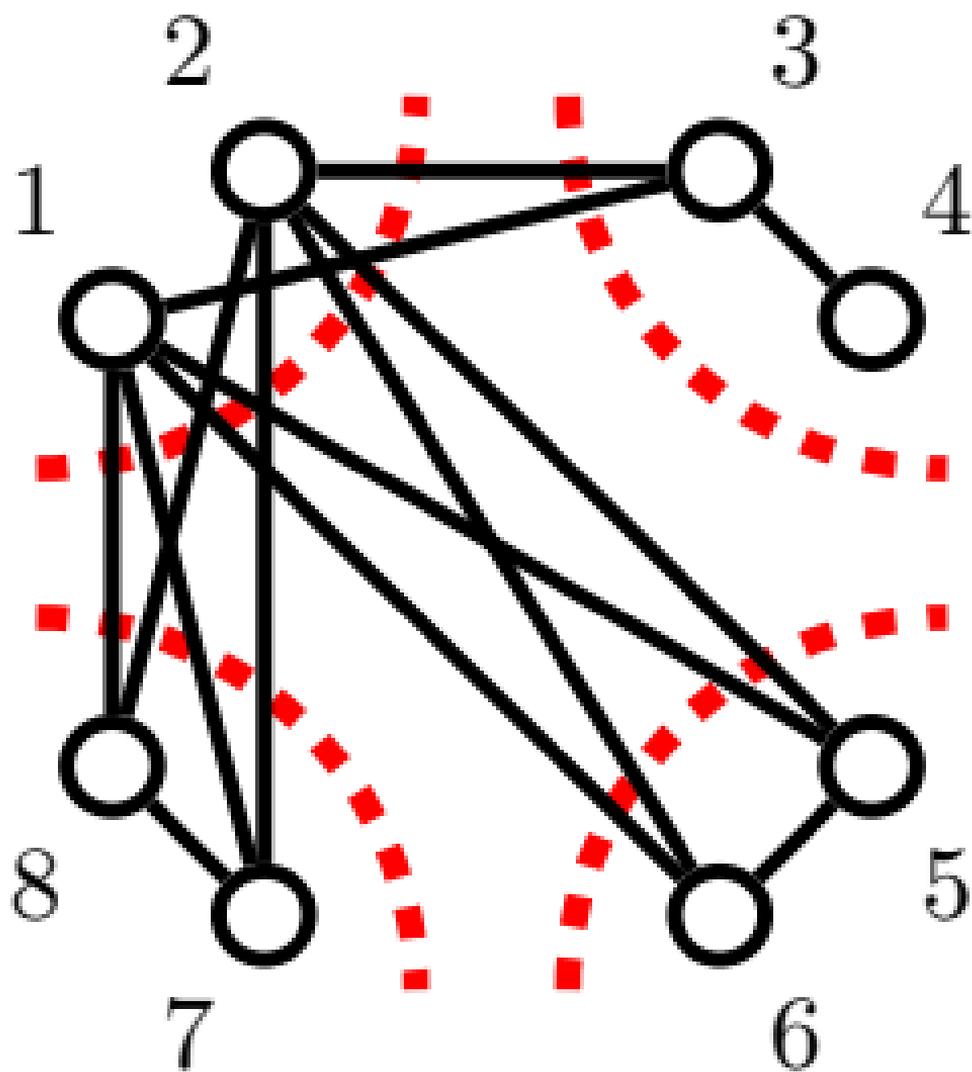

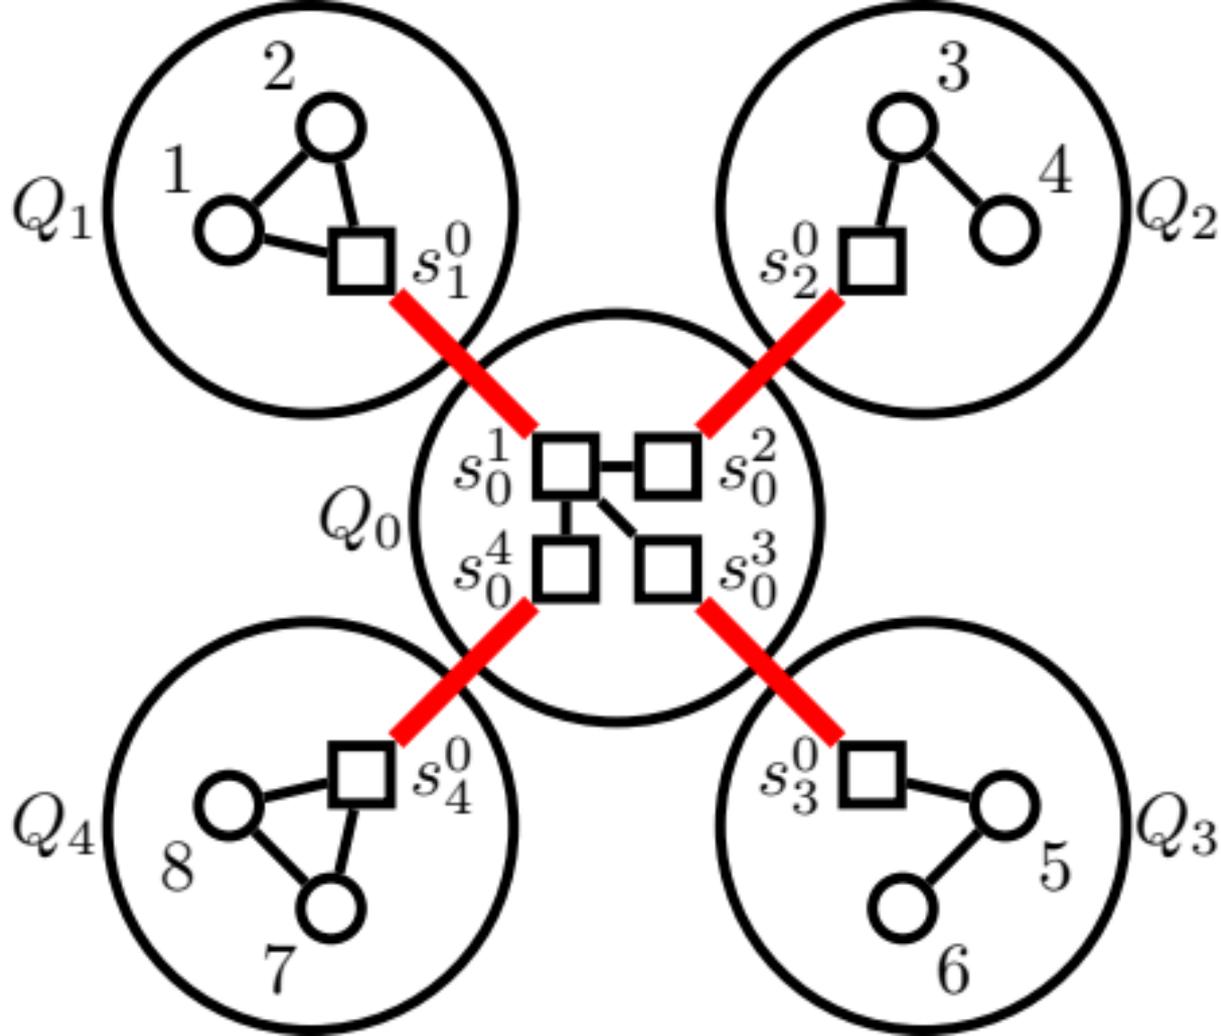



$K_{2,2,2,2}$ 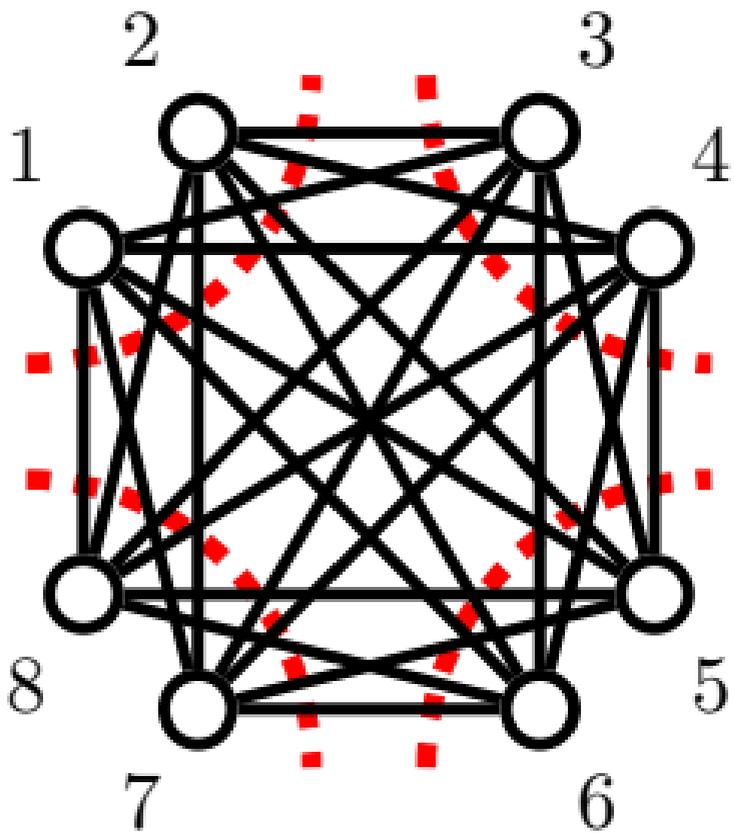 $ep(5, 7) \circ ep(1, 3)$ 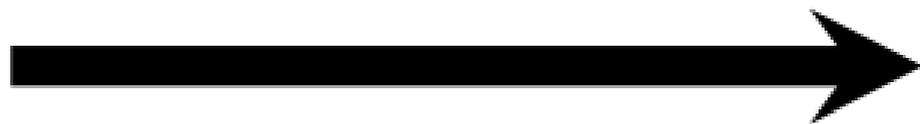 $R_4$ 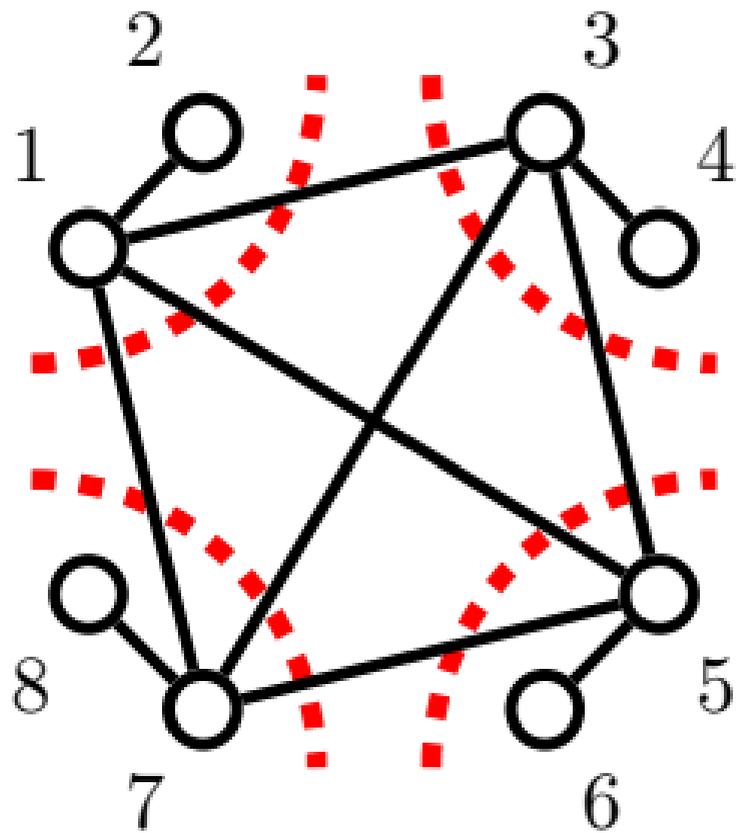

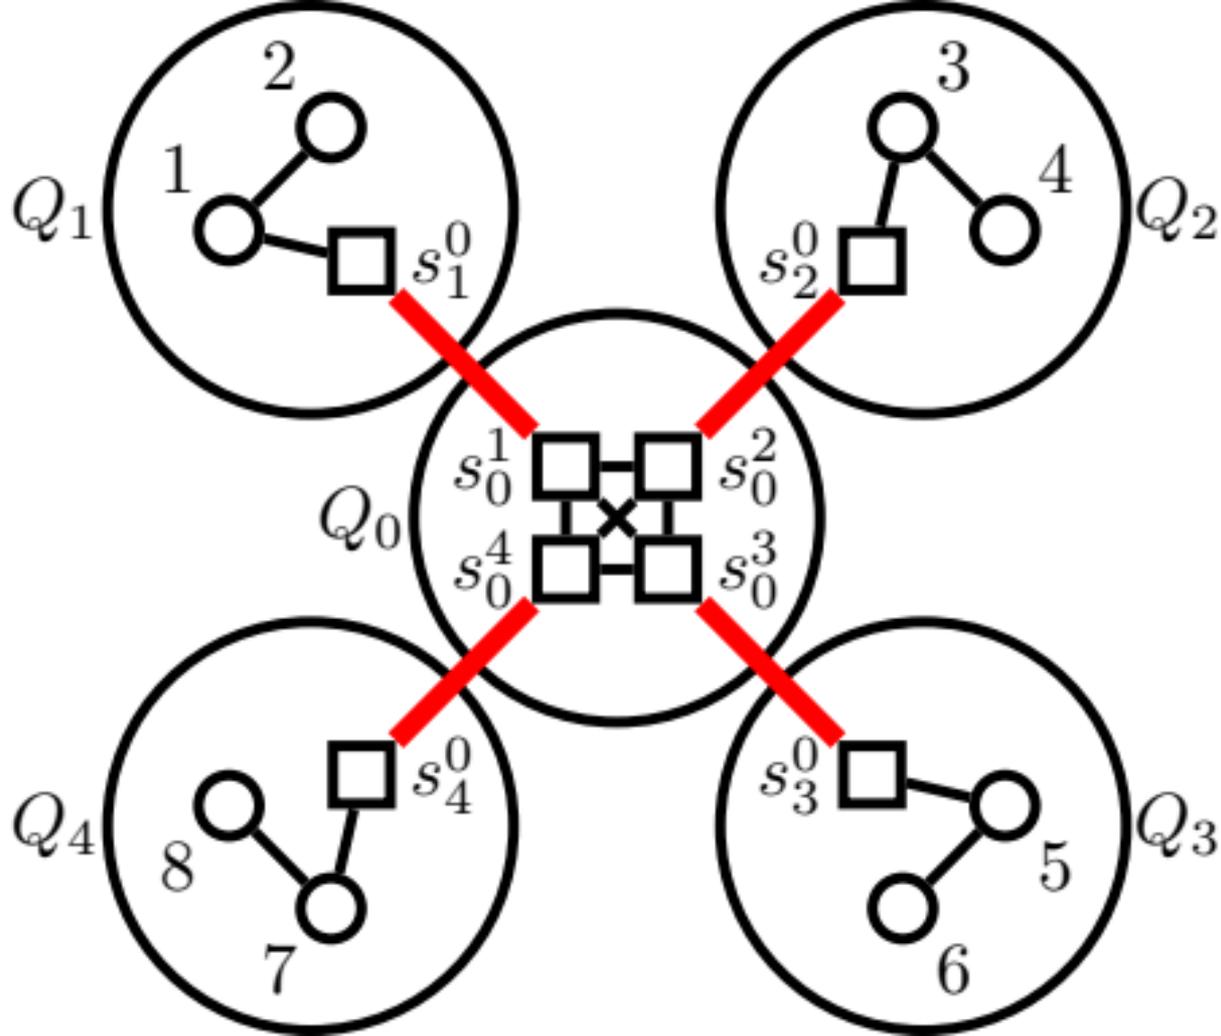

$CS_{2,2,2}^1$ 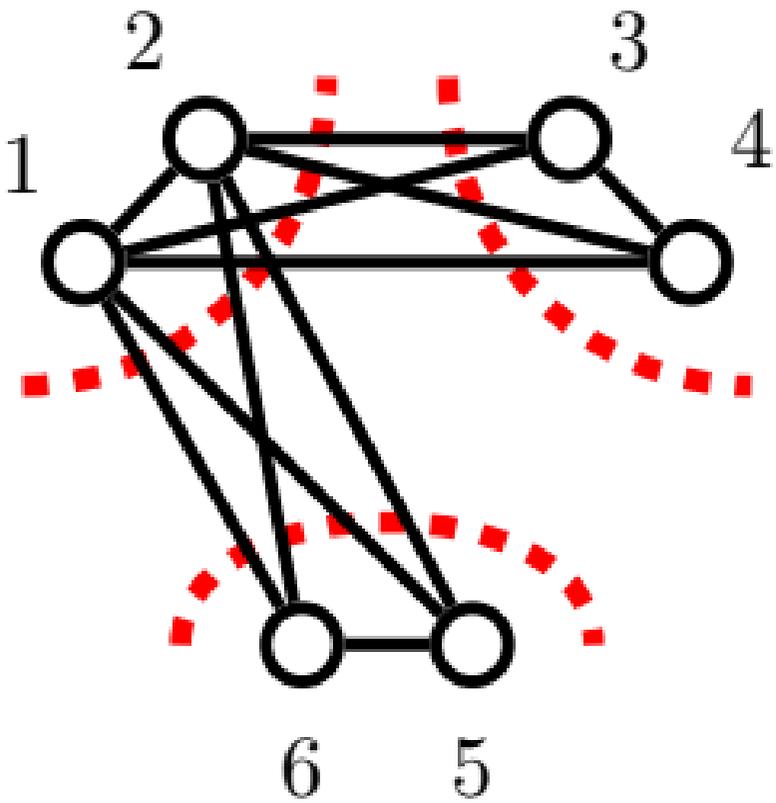 $C_1 \circ C_5 \circ C_3$ 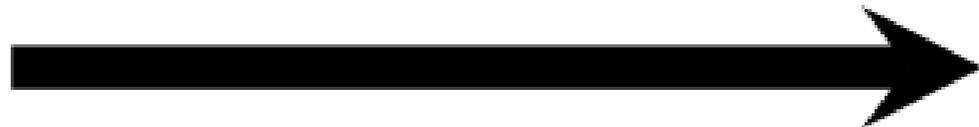 $R_3$ 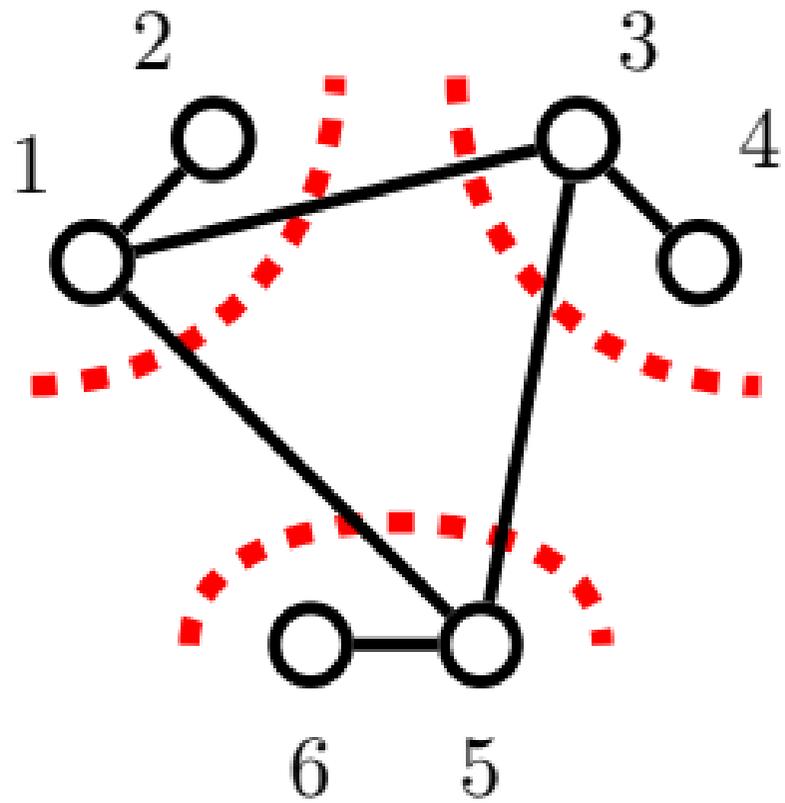

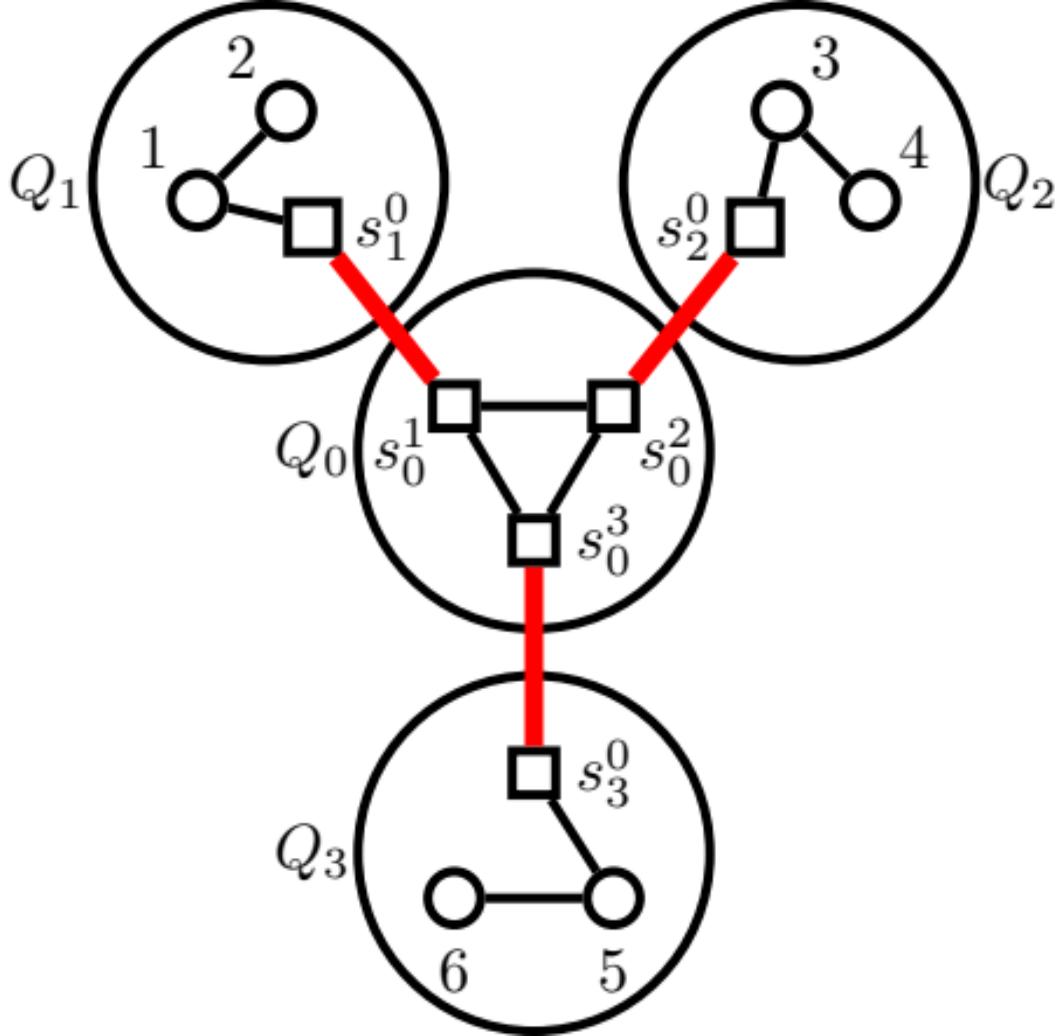

Case 1

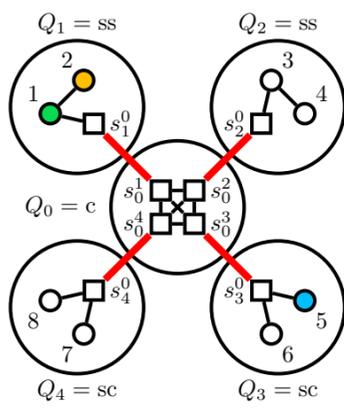
 $c_1$   
1-a

 $c_5$   
1-c

 $c_2$  1-b
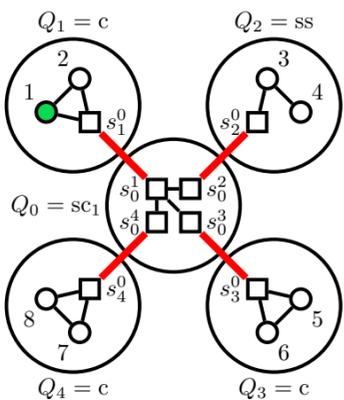

Case 3

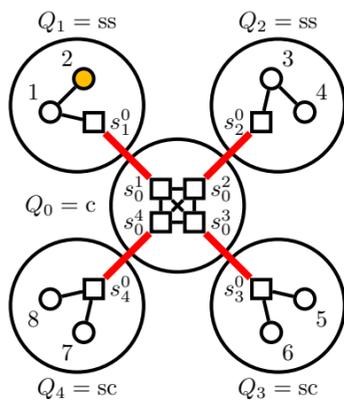

Case 1

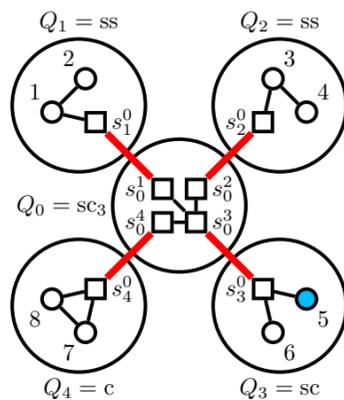

Case 2

Case 2

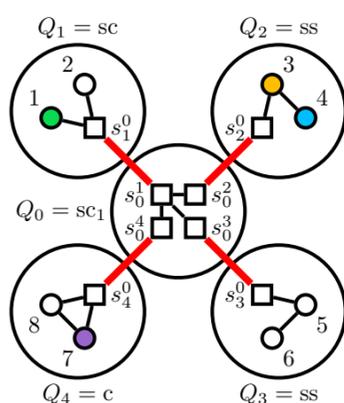
 $c_1$   
2(j)-a

 $c_4$   
2(j)-c

 $c_3$  2(j)-b

 $c_7$  2(j)-d
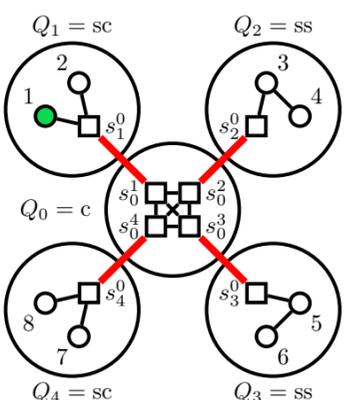

Case 1

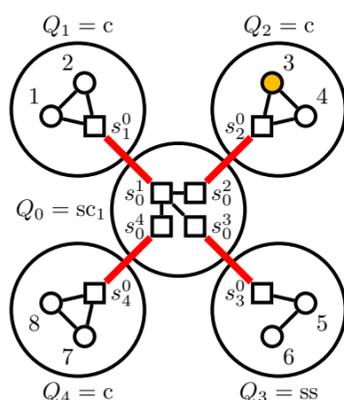

Case 3

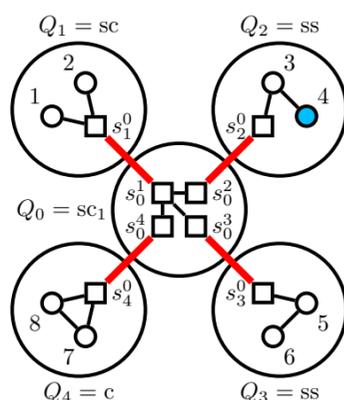

Case 2

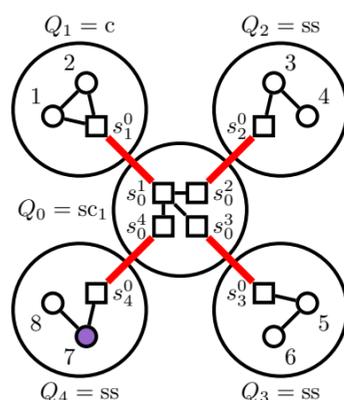

Case 3

Case 3

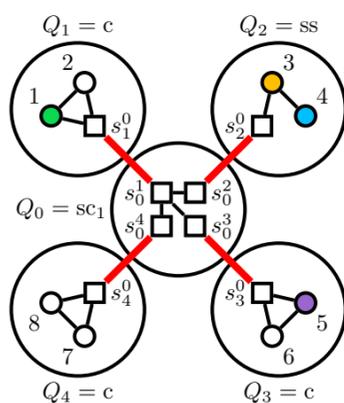
 $c_1$   
3(j)-a

 $c_4$   
3(j)-c

 $c_3$  3(j)-b

 $c_5$  3(j)-d
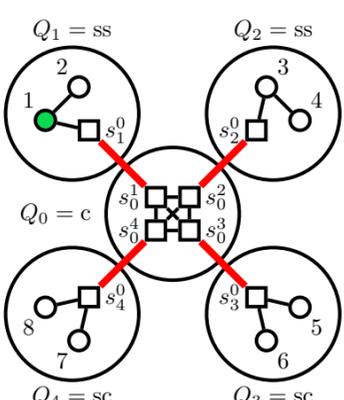

Case 1

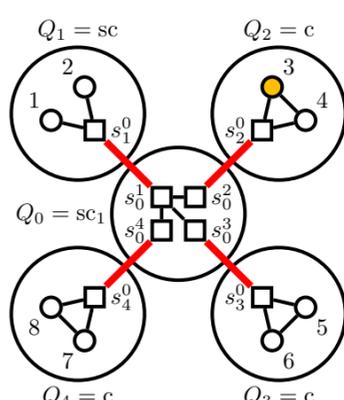

Case 2

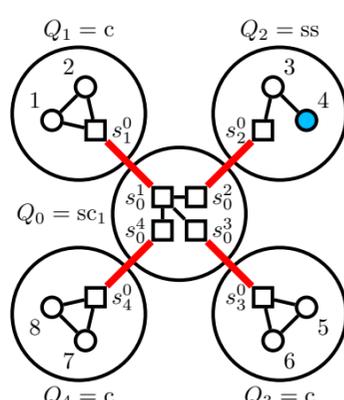

Case 3

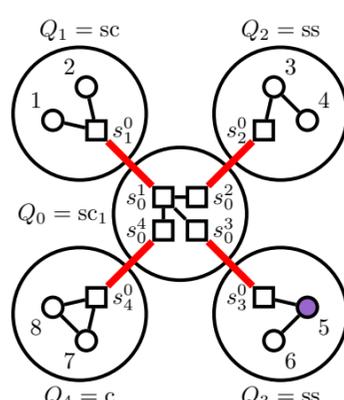

Case 2
