# Supplementary material for: Local Equivalence Classes of Distance-Hereditary Graphs using Split Decompositions
Source: arXiv:2602.23825 source file (2026-02-27)

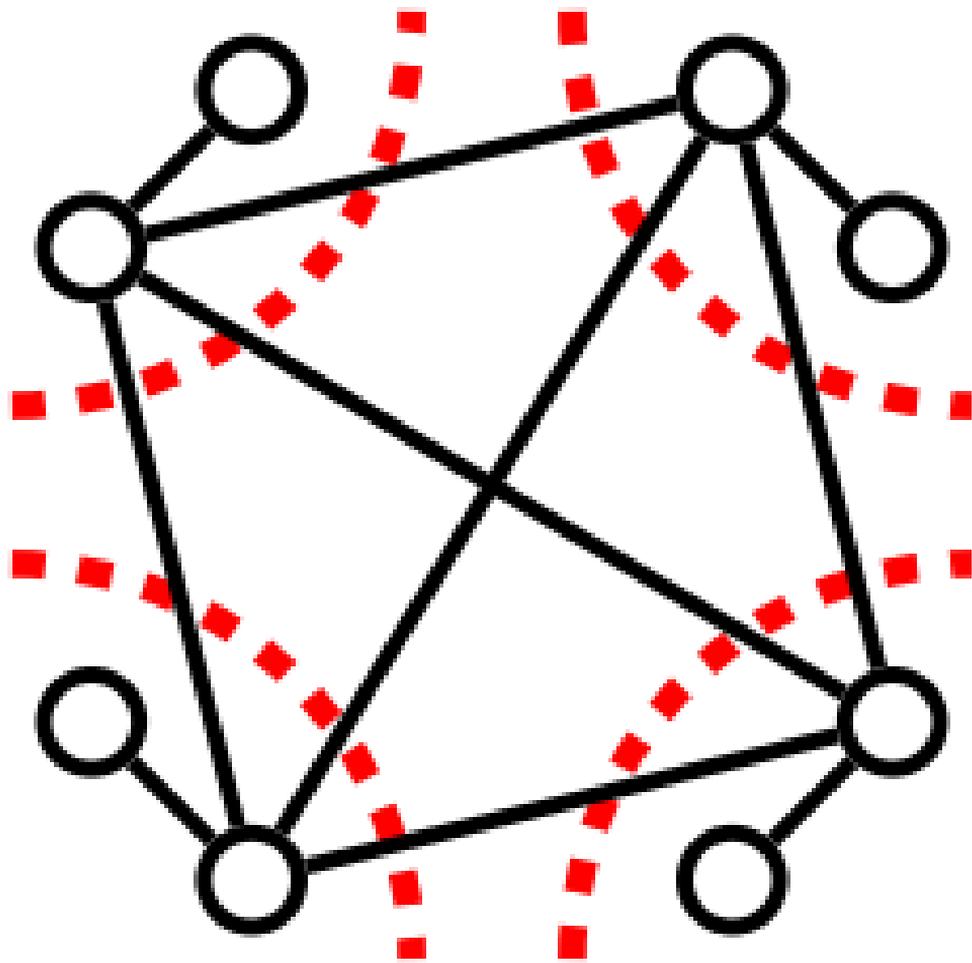

$G_1$

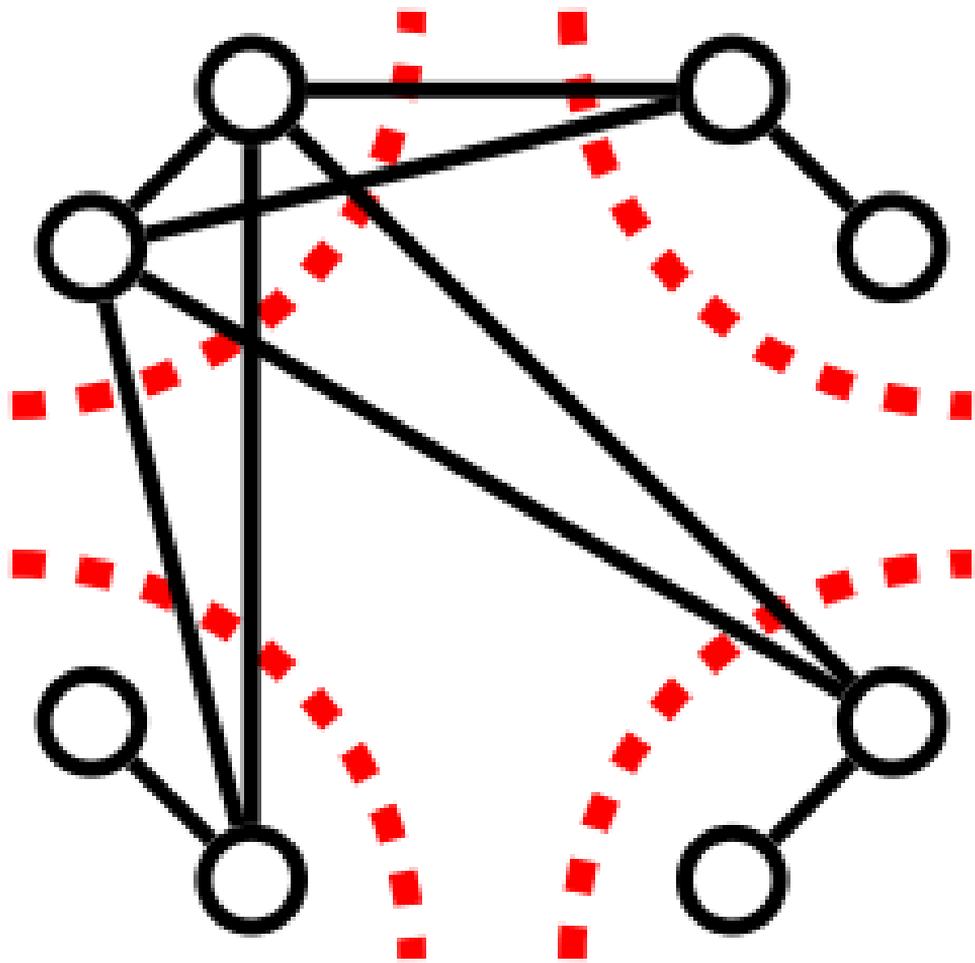

$G_3$

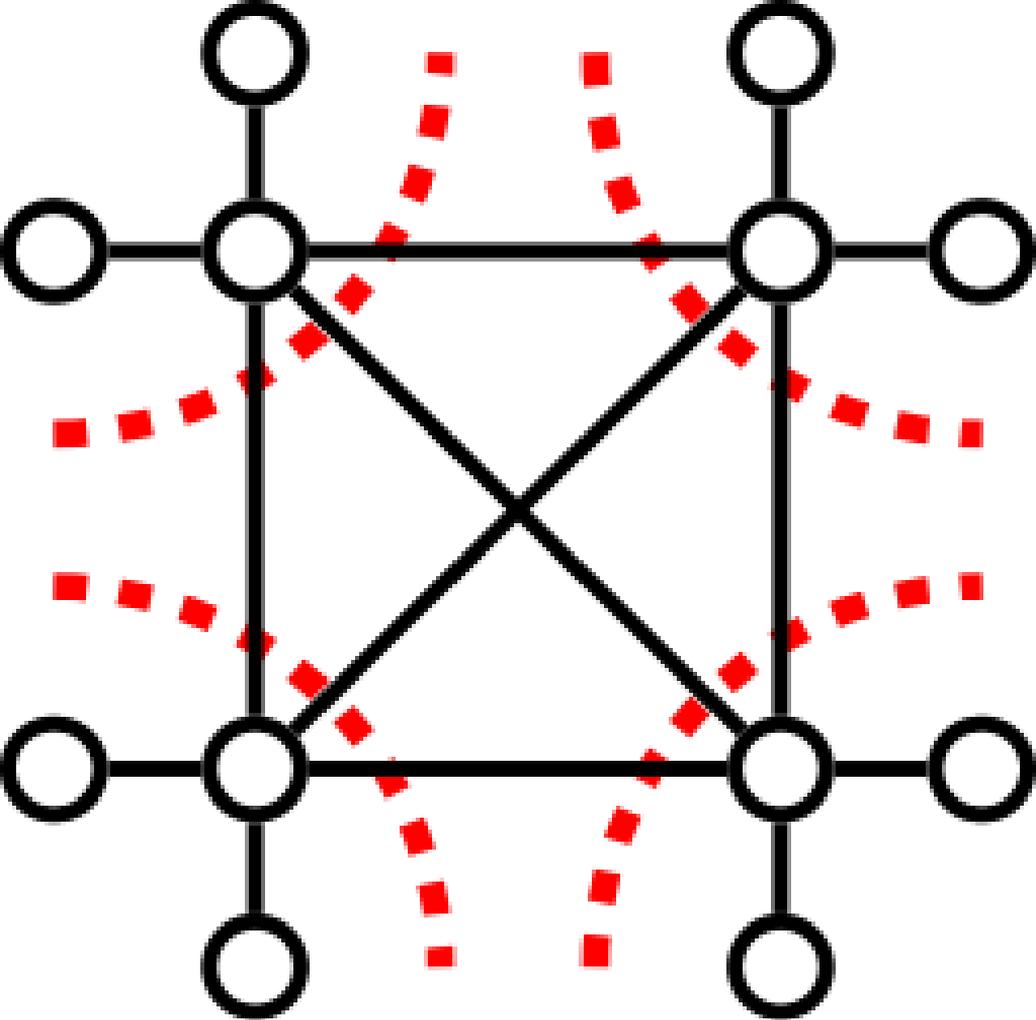

$G_1$

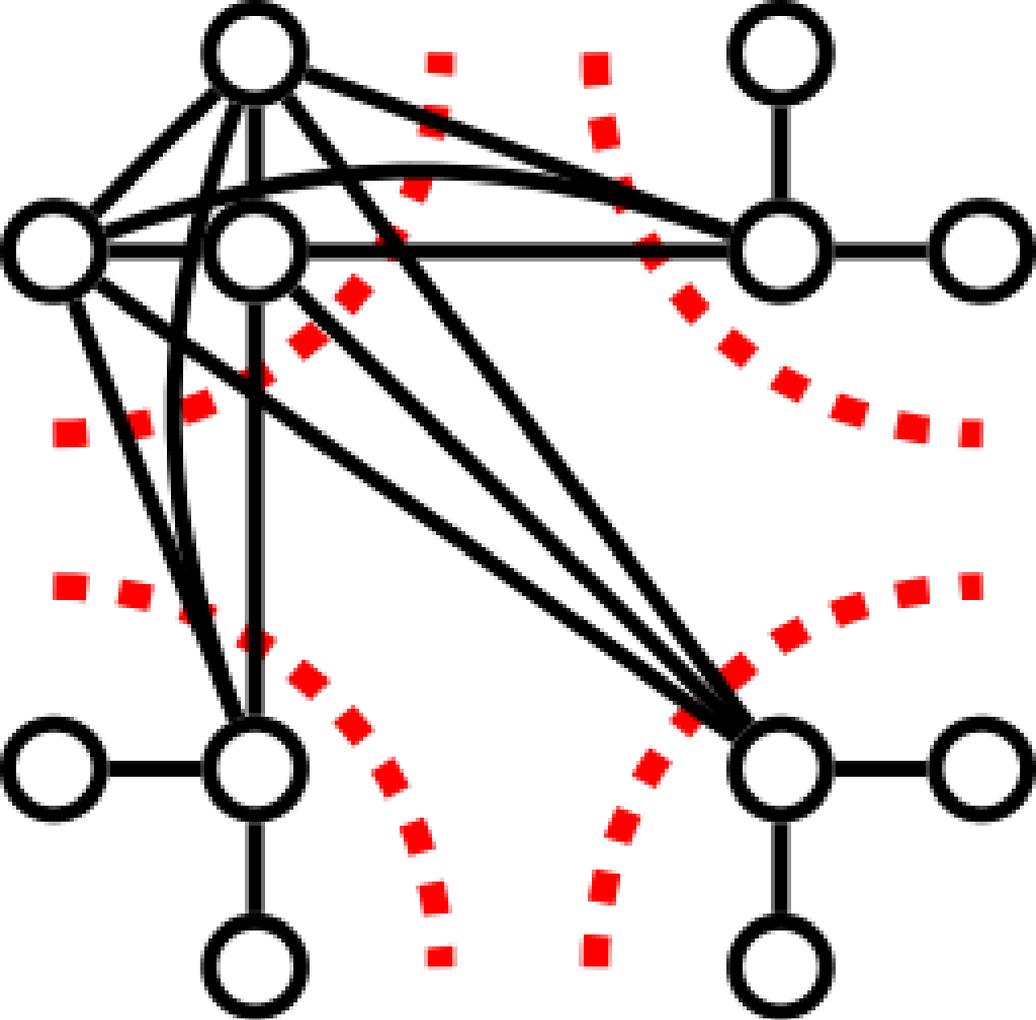

$G_3$

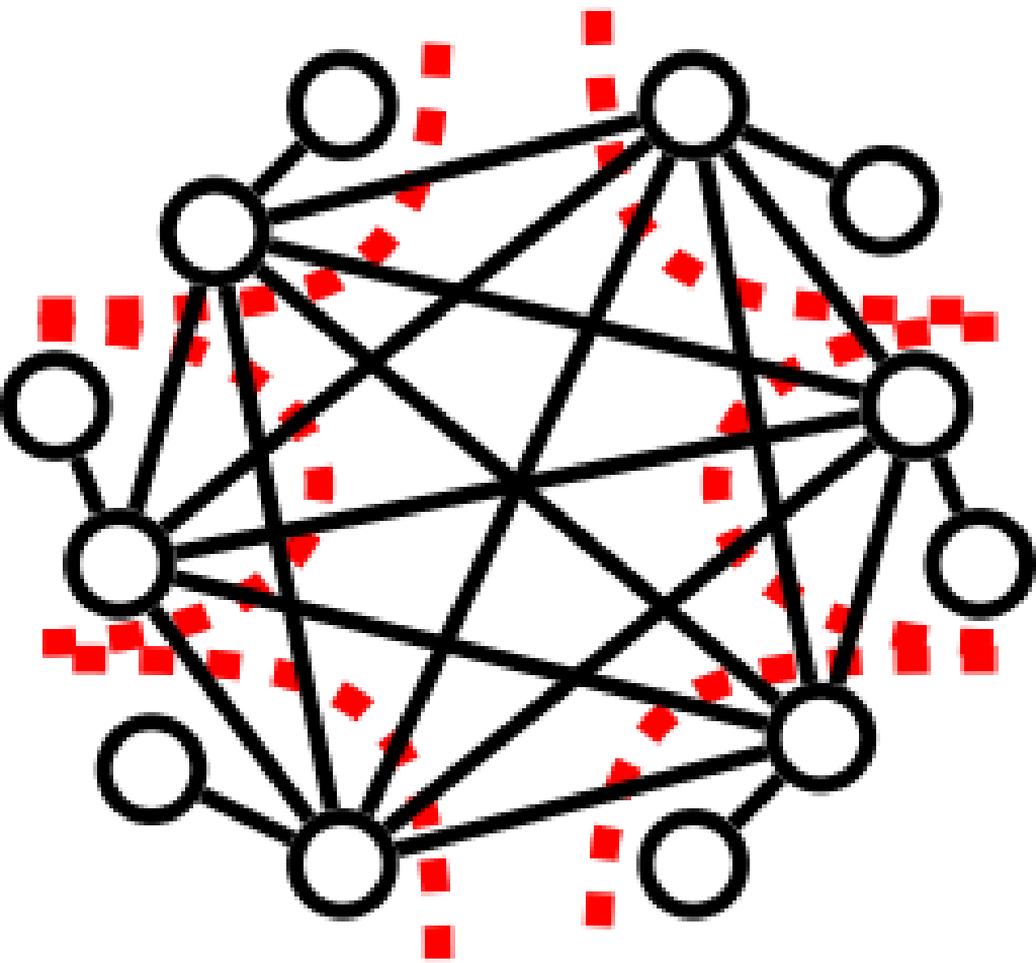

$G_1$

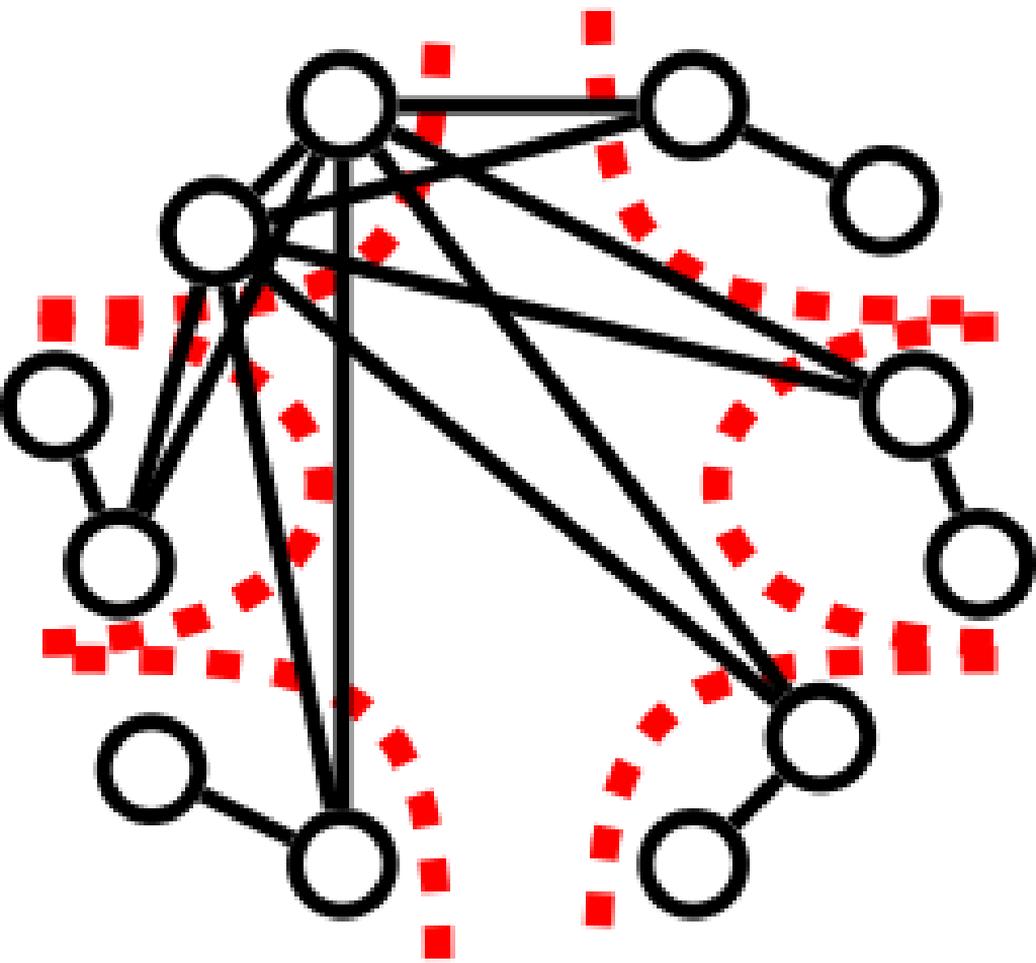

$G_3$

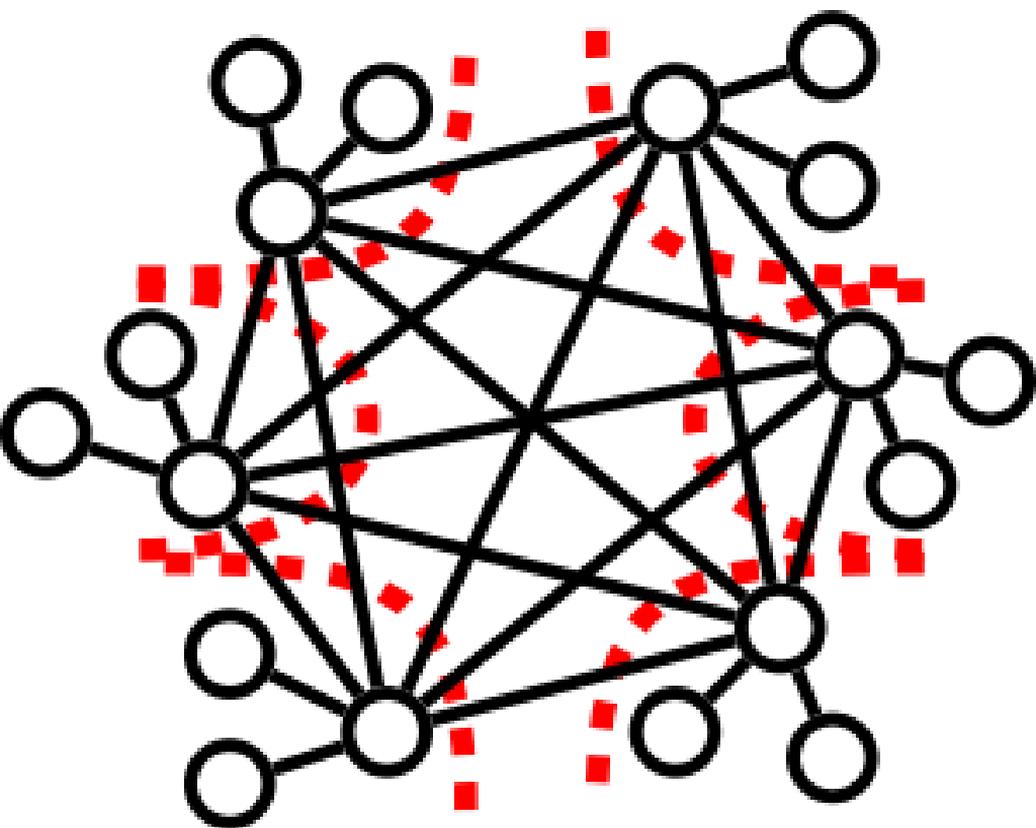

$G_1$

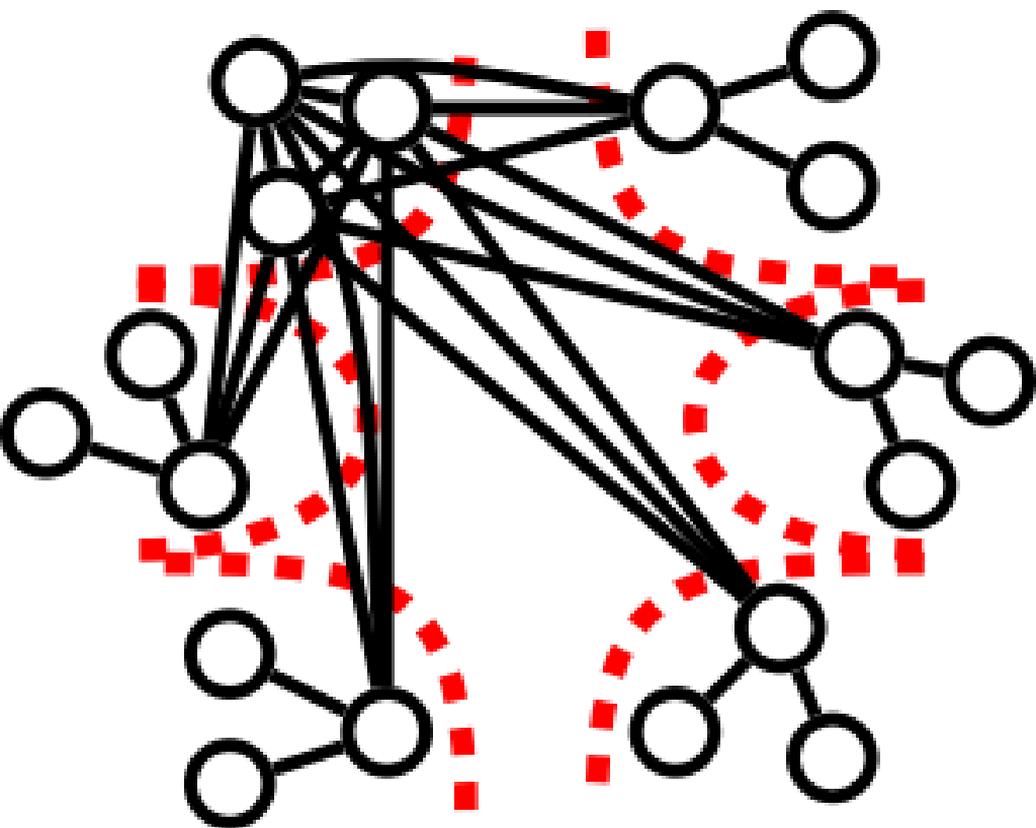

$G_3$

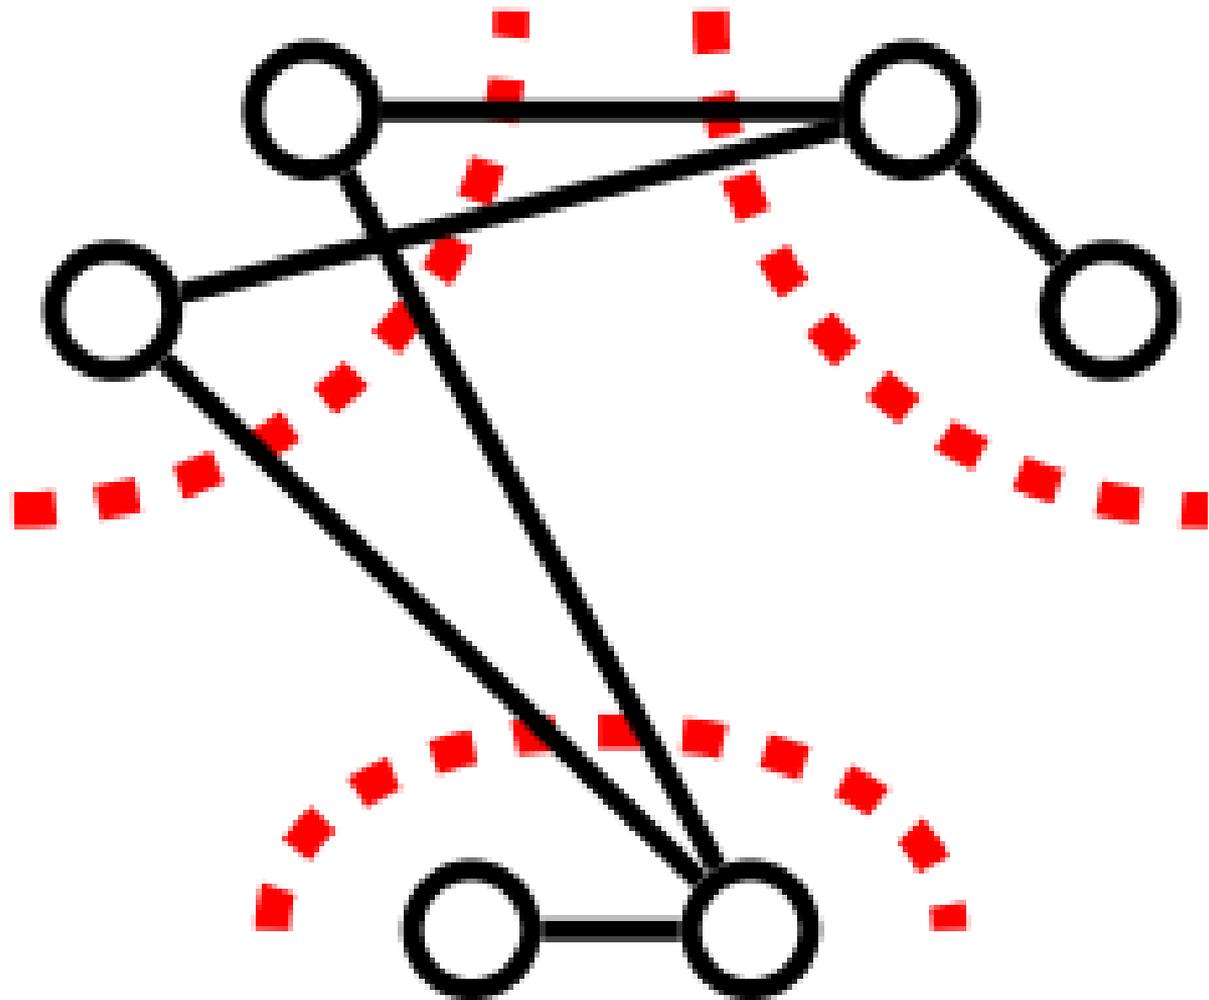

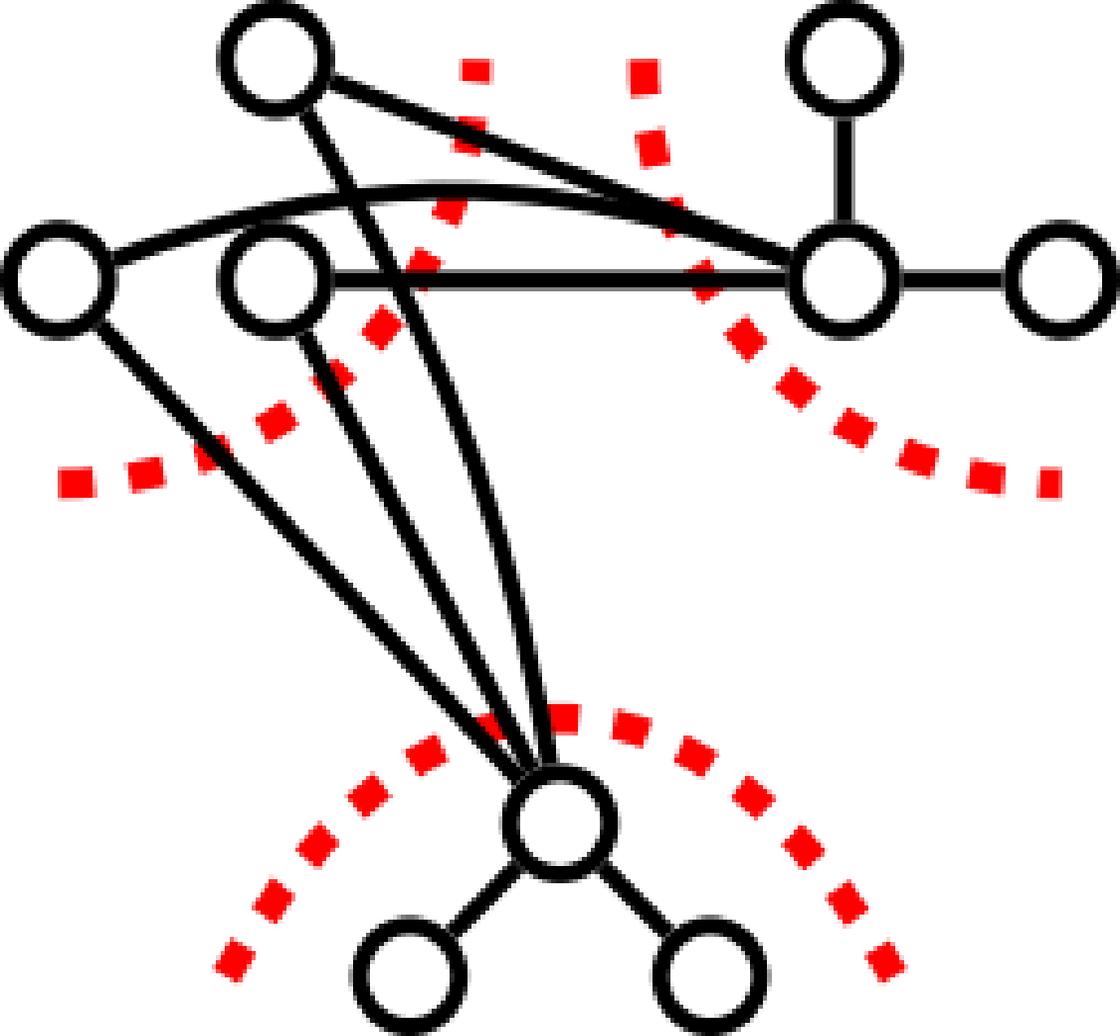

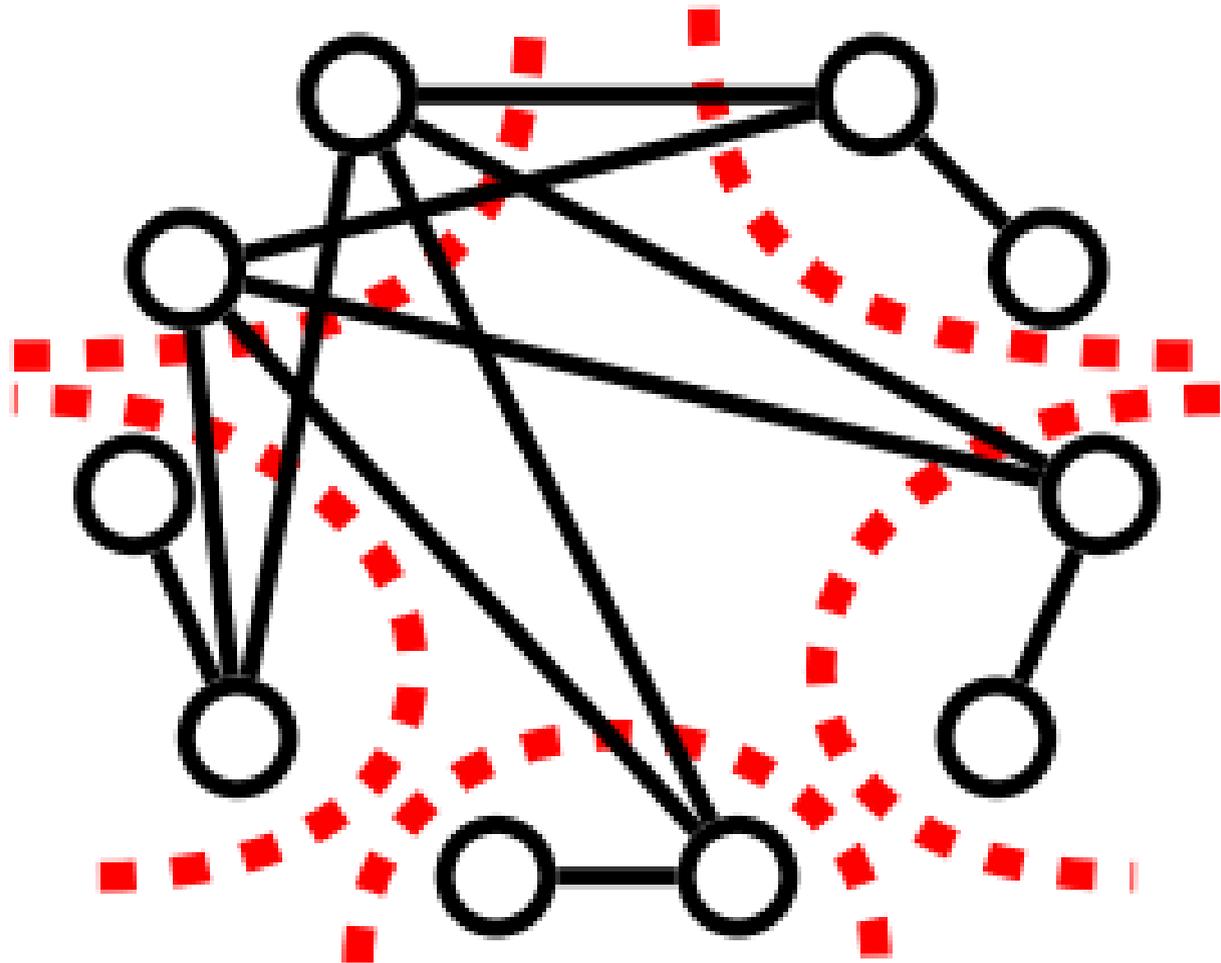

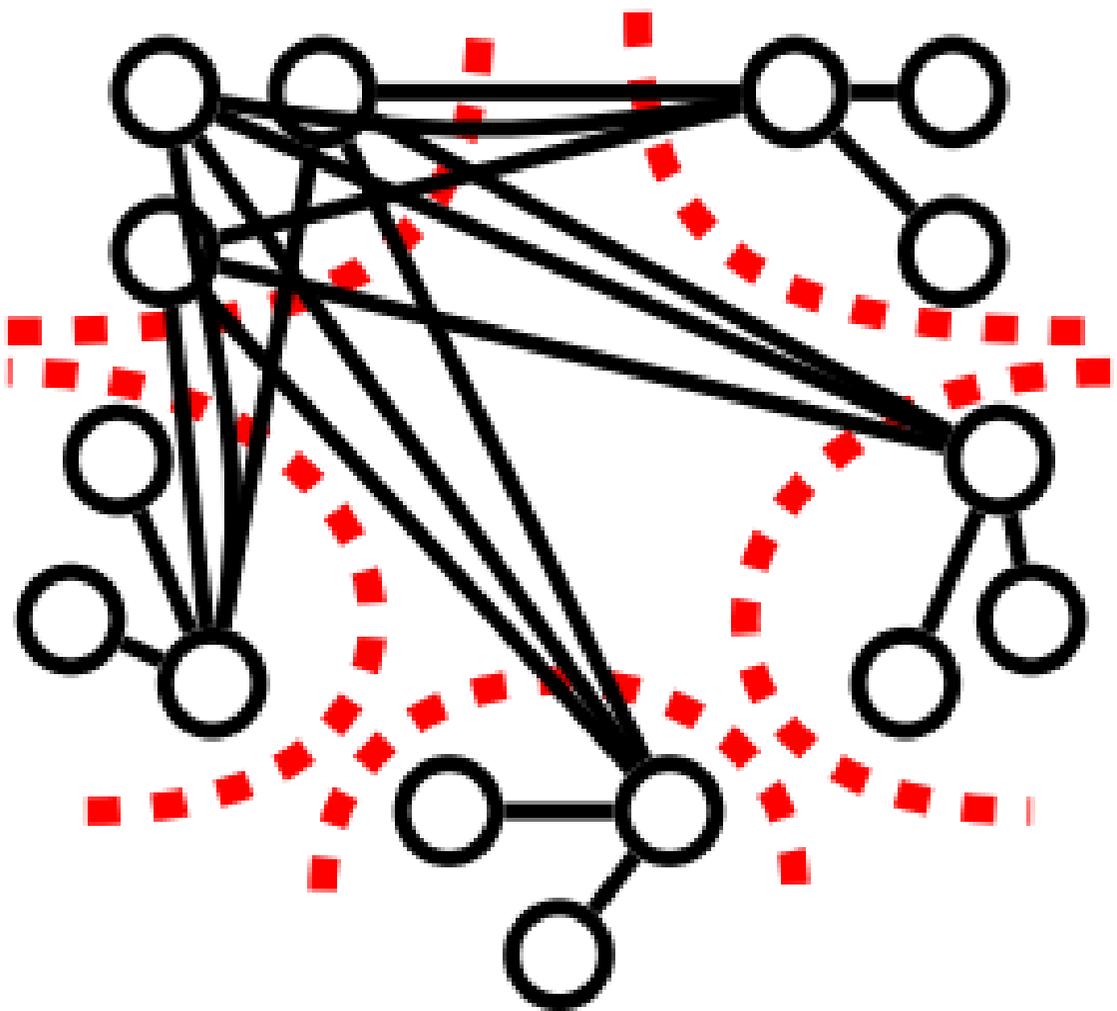

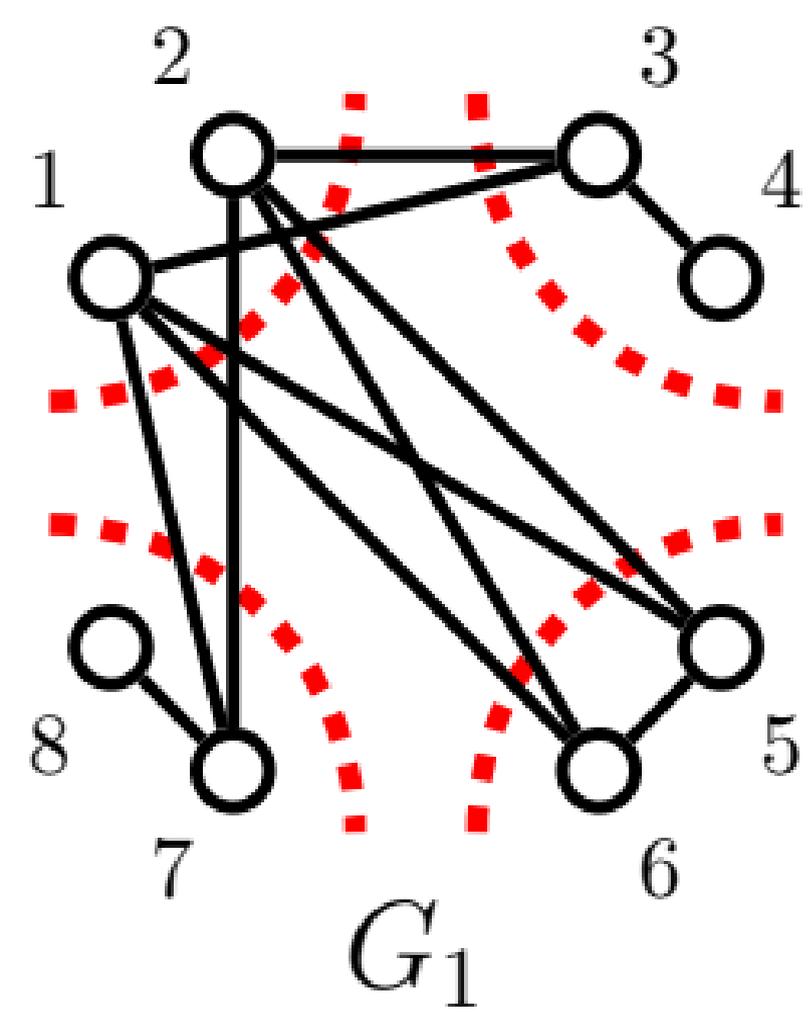

$\cong$

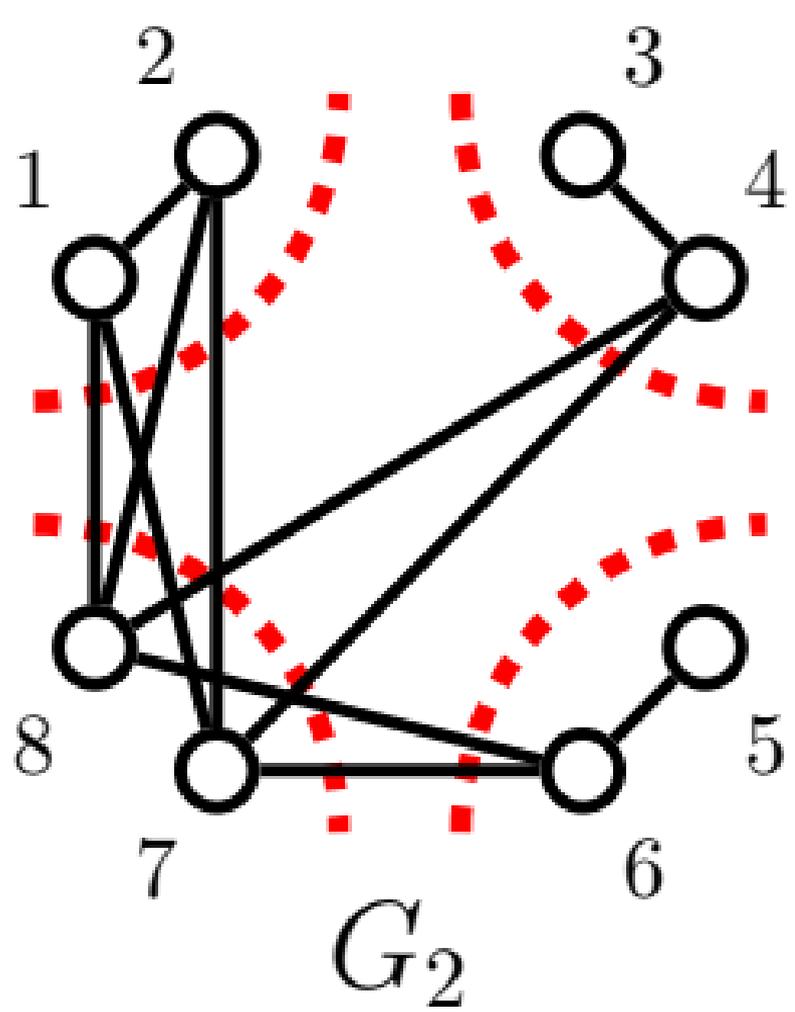

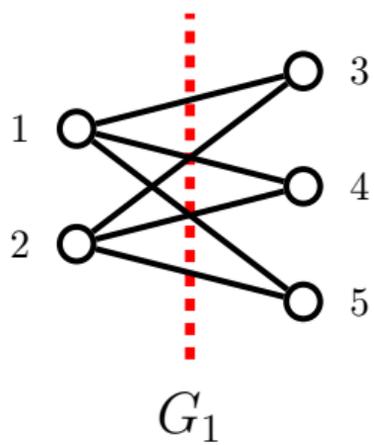

$\cong$

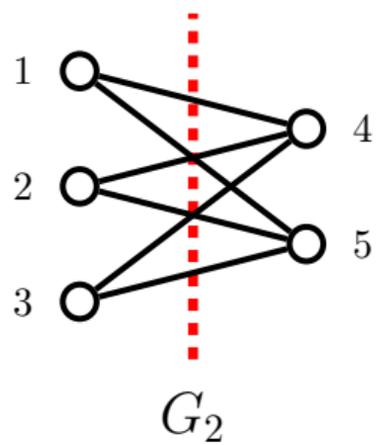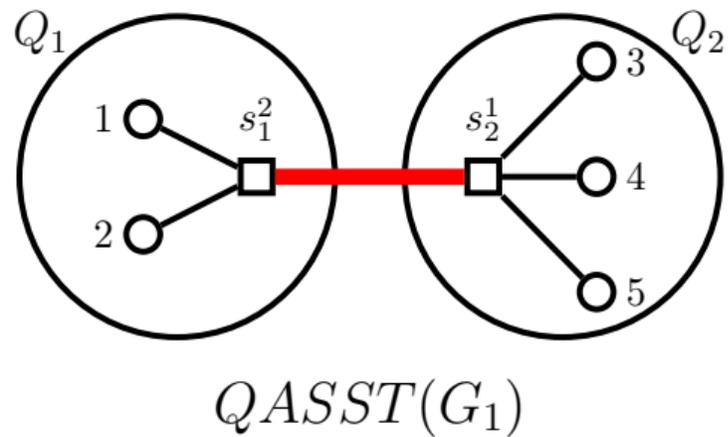

$\not\cong_{LC}$

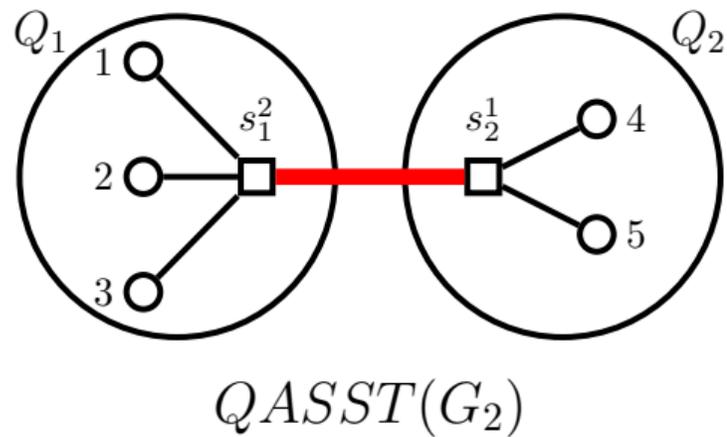

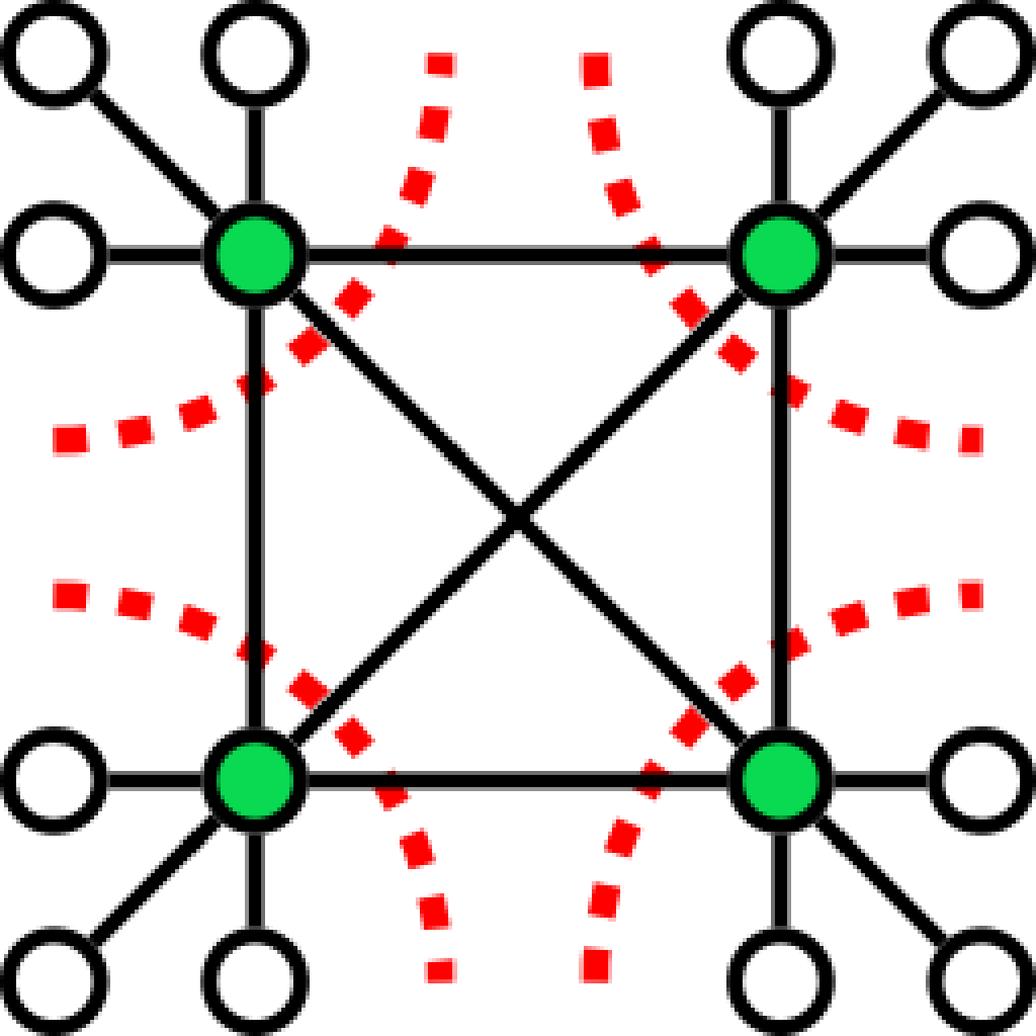

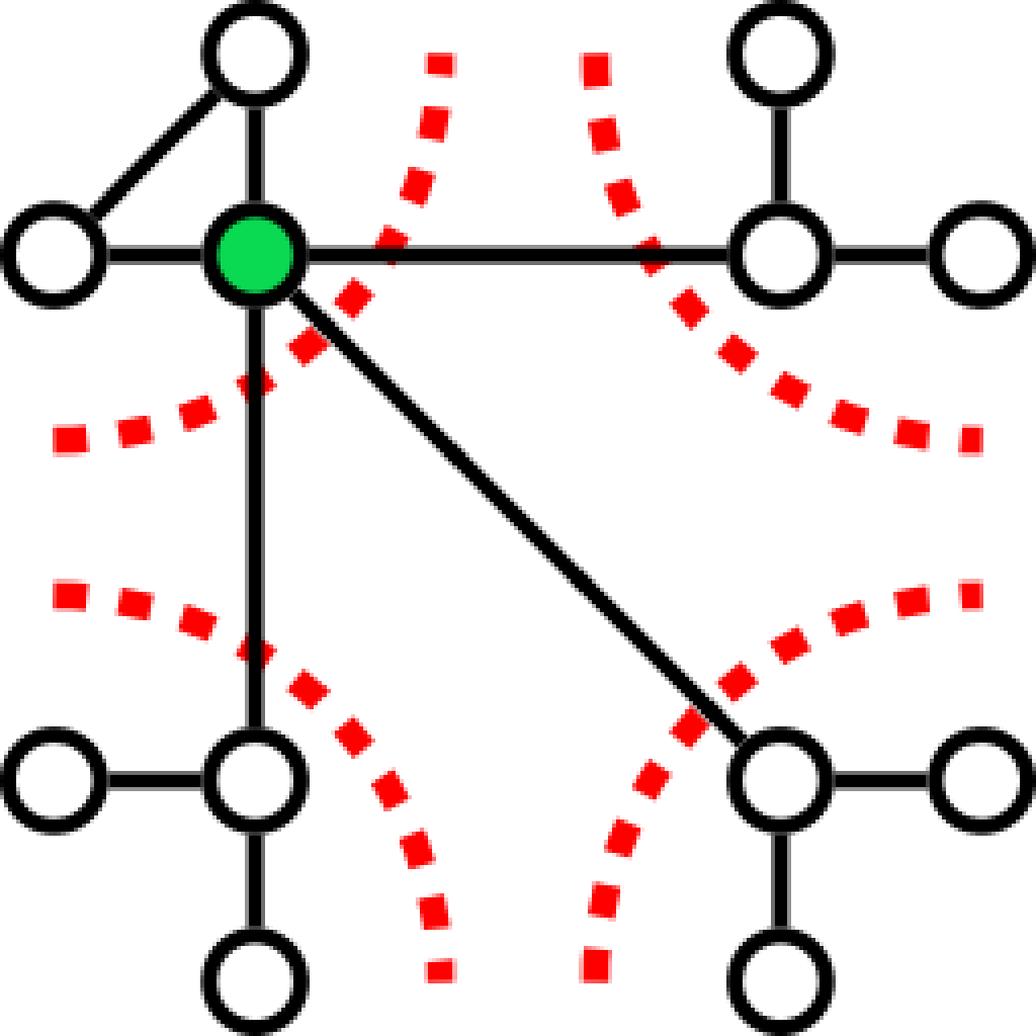

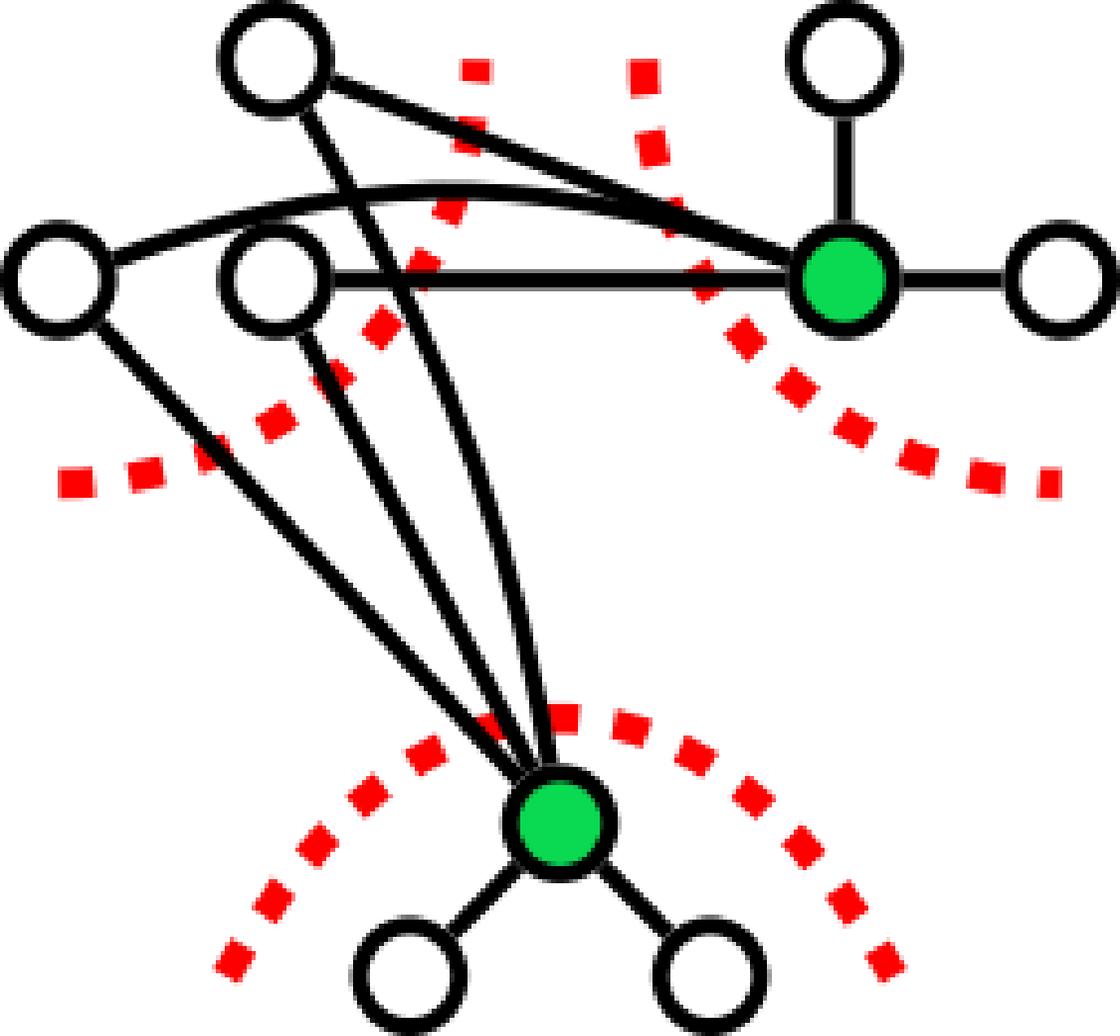

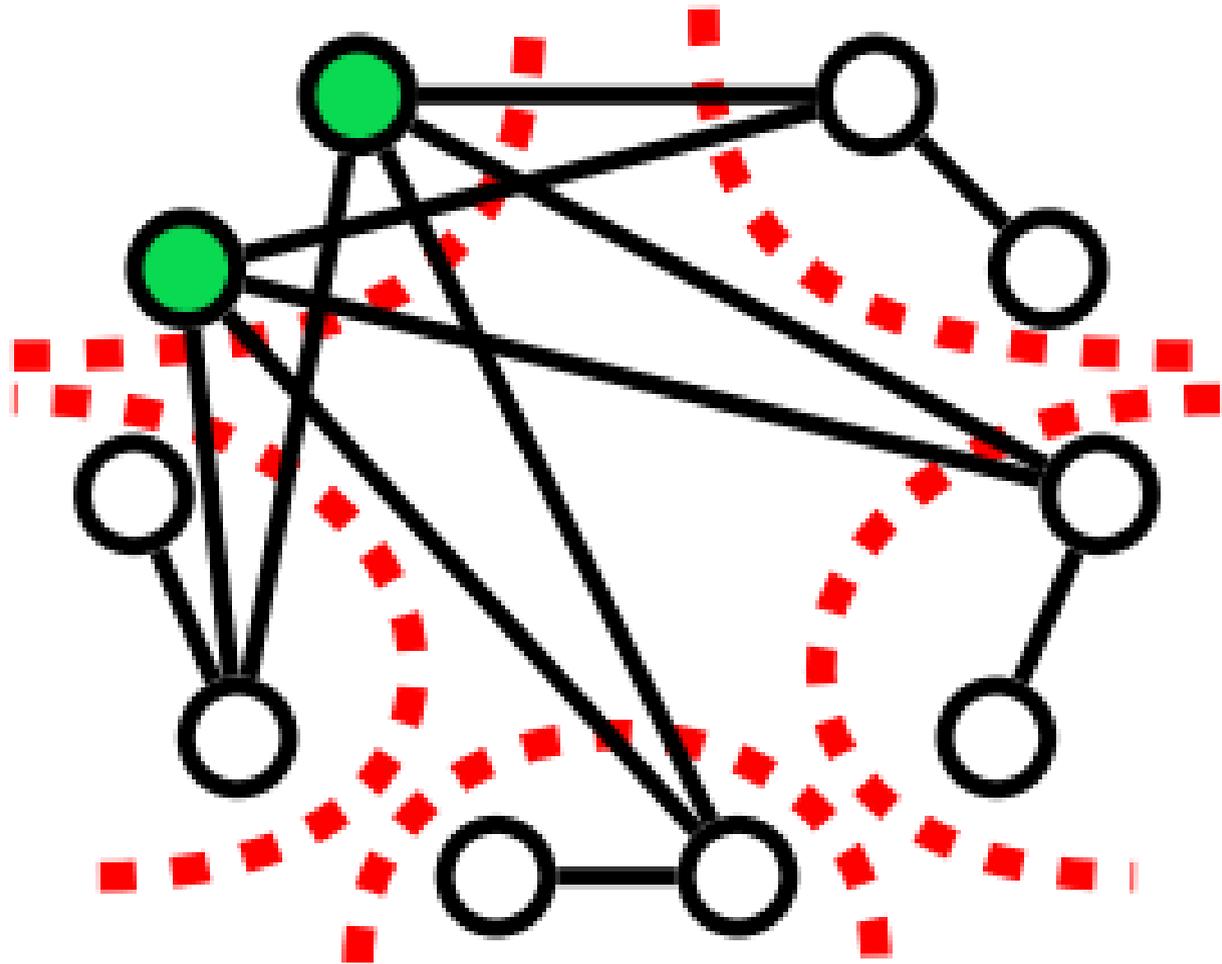

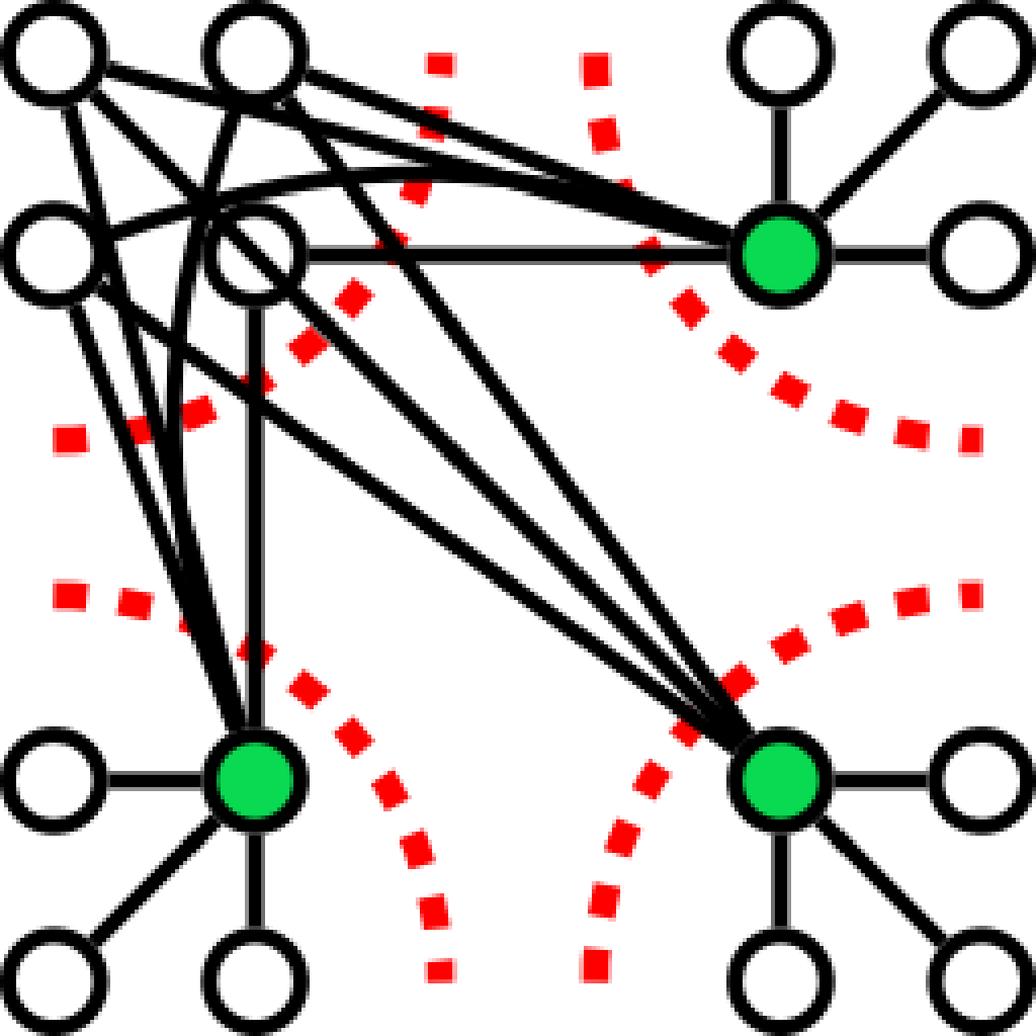

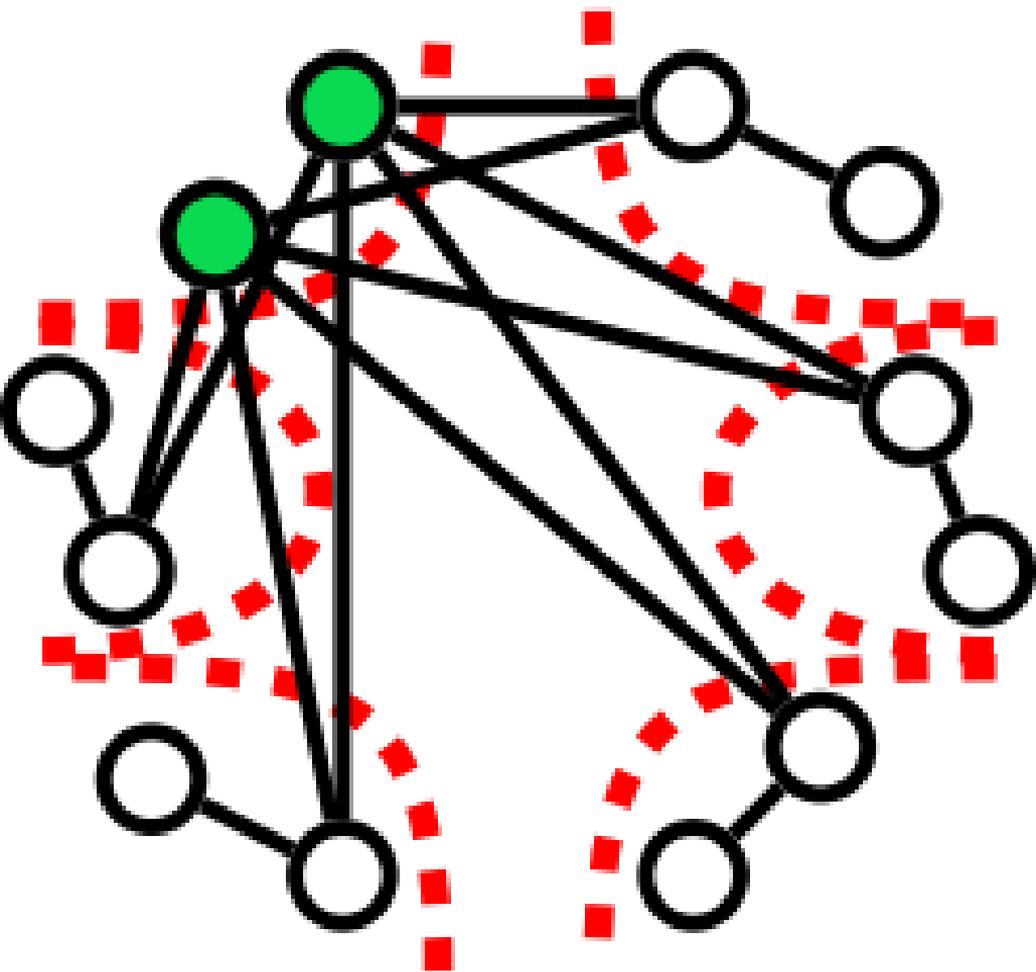

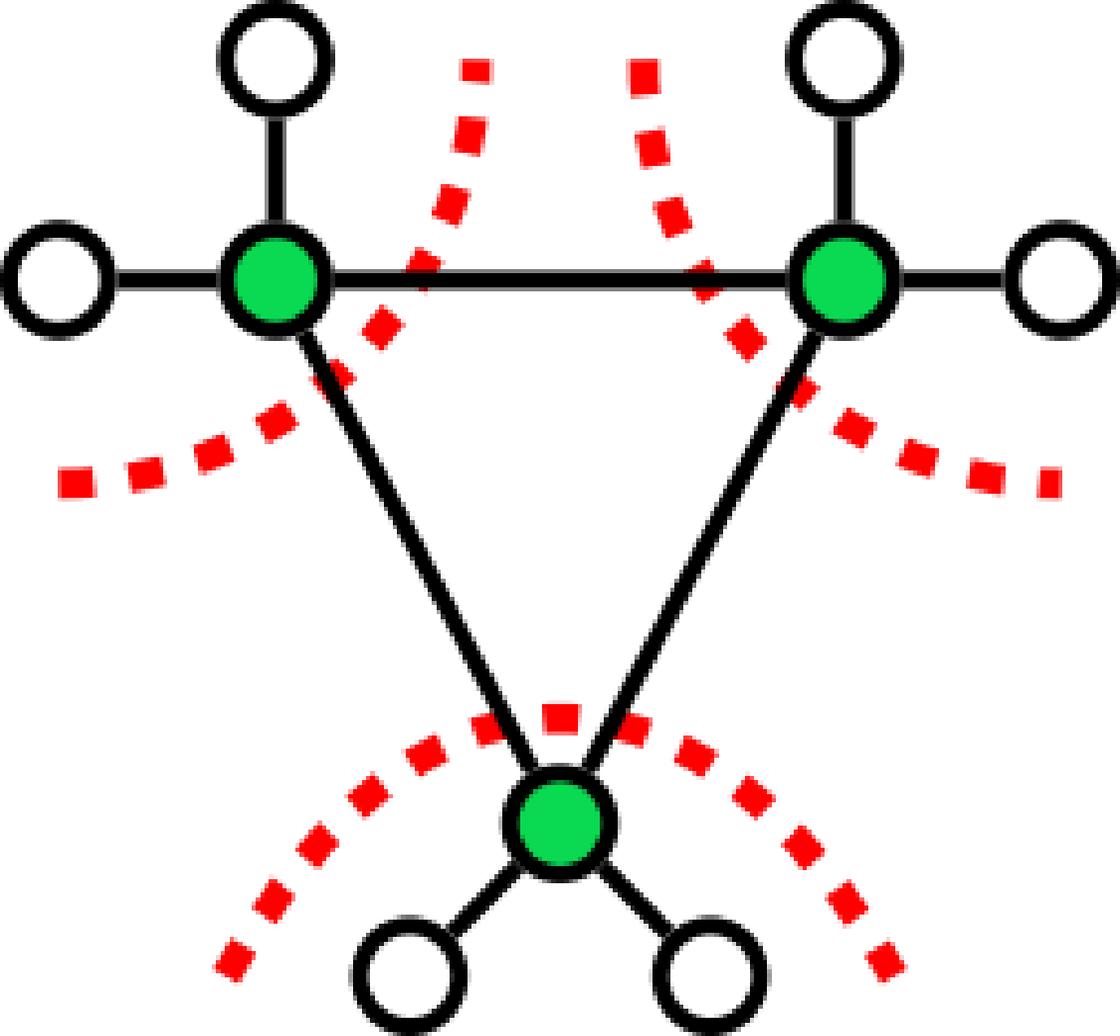

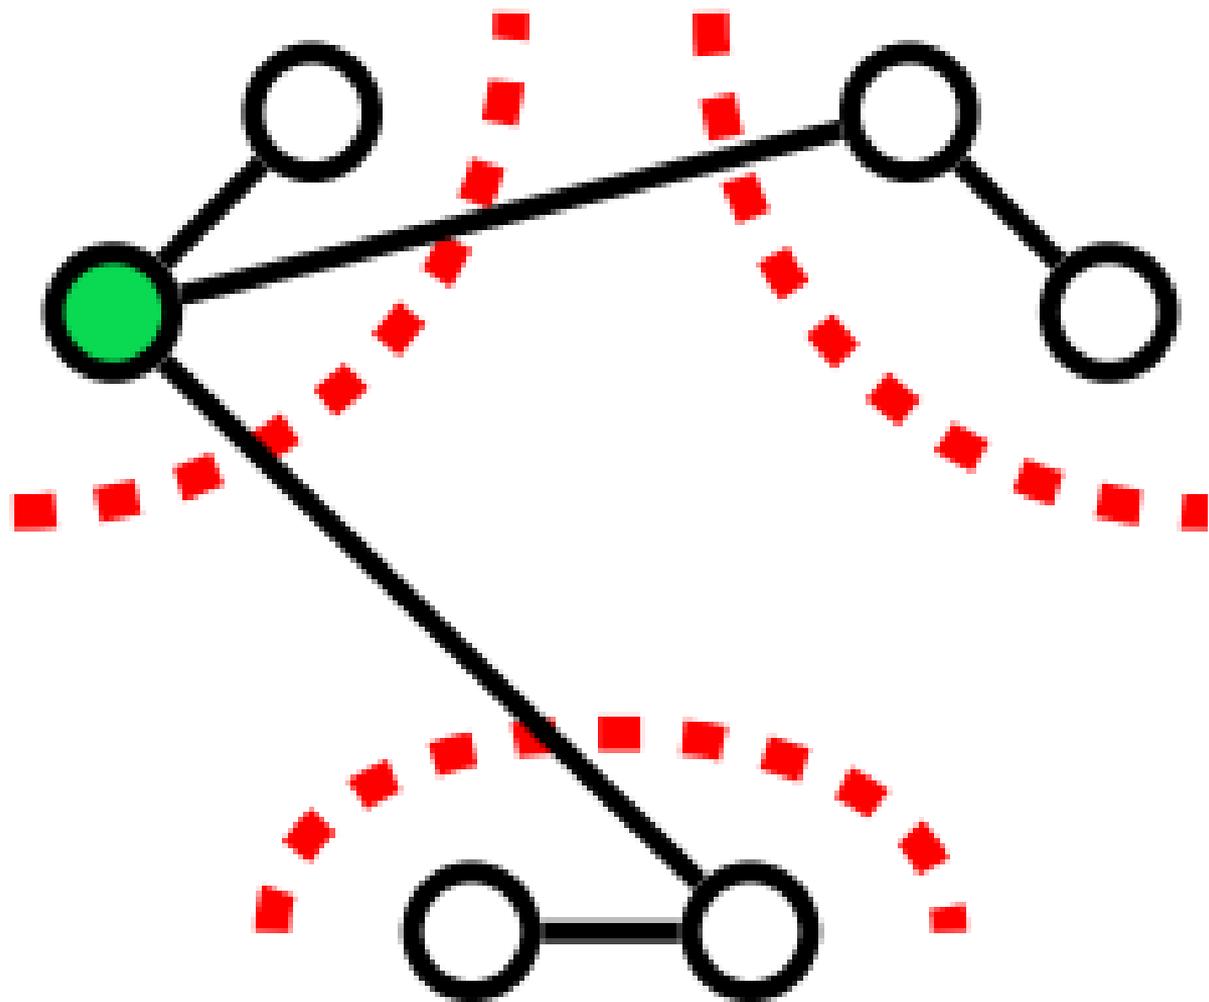

Supplement: Supplementary file 2 [file Appendix_Edge_Counting_and_Isomorphisms.pdf]
